# Supplementary material for: Marrying critical oscillators with traveling waves shapes nonlinear sound processing in the cochlea
Source: arXiv:2512.11646 ancillary file (2025-12-15)
Supplement: Supplementary file 1 [file supplement.pdf]

1

## 2 Supplemental Material for

3 **Marrying critical oscillators with traveling waves**  
4 **shapes nonlinear sound processing in the cochlea.**

5 **Henri Ver Hulst, Carles Blanch Mercader, Frank Jülicher and Pascal Martin\***

6

7 **Contact author: [pascal.martin@curie.fr](mailto:pascal.martin@curie.fr)**

### **This PDF file includes:**

8

Supplemental Data (Figs. S1 to S4)

9

Supplemental Text with Tables S1 to S2 and Figures S5 to S11

10

SM References

11

## 12 Contents

|    |          |                                                                                      |           |
|----|----------|--------------------------------------------------------------------------------------|-----------|
| 13 | <b>A</b> | <b>Supplementary Data (Figs. S1-S4)</b>                                              | <b>3</b>  |
| 14 | <b>B</b> | <b>Definition and generic properties of a critical oscillator.</b>                   | <b>7</b>  |
| 15 | 1        | Response to a sinusoidal stimulus near a Hopf bifurcation—critical slowing down . .  | 7         |
| 16 | 2        | Linear response and energy pumping . . . . .                                         | 10        |
| 17 | <b>C</b> | <b>Box model of the cochlea based on critical oscillators</b>                        | <b>13</b> |
| 18 | 1        | Description of the partition as a chain of critical oscillators . . . . .            | 13        |
| 19 | 2        | Box model with two-dimensional hydrodynamics . . . . .                               | 14        |
| 20 | 3        | Box model with one-dimensional hydrodynamics . . . . .                               | 16        |
| 21 | 4        | Pure-tone stimulus to the box model . . . . .                                        | 17        |
| 22 | 5        | Output of the model: Response of the oscillators, driving pressure and energy flux . | 18        |
| 23 | <b>D</b> | <b>Methods to solve the model</b>                                                    | <b>19</b> |
| 24 | 1        | Solution for the pressure field using the Green-function method . . . . .            | 19        |
| 25 | 2        | Numerical resolution of the model . . . . .                                          | 22        |
| 26 | 2.a      | With 2D hydrodynamics . . . . .                                                      | 22        |
| 27 | 2.b      | With 1D hydrodynamics . . . . .                                                      | 24        |
| 28 | 2.c      | Discretization of space and time . . . . .                                           | 25        |
| 29 | 2.d      | Computation of the energy flux . . . . .                                             | 25        |
| 30 | 2.e      | Frequency-tuning curve of sensitivity . . . . .                                      | 26        |
| 31 | 3        | Confronting numerical results of the model to experiments: matching procedure . .    | 27        |
| 32 | 4        | Parameter values and methodology for each numerical implemetation of the model       |           |
| 33 |          | (with Tables S1 and S2) . . . . .                                                    | 29        |
| 34 | <b>E</b> | <b>Analytical solution of the model under the WKB approximation</b>                  | <b>30</b> |
| 35 | 1        | Dispersion relation, pressure field and energy flux with 2D hydrodynamics . . . . .  | 30        |
| 36 | 2        | Dispersion relation, pressure field and energy flux with 1D hydrodynamics . . . . .  | 31        |
| 37 | <b>F</b> | <b>Mapping between the linearized Hopf normal form and the local equation of</b>     |           |
| 38 |          | <b>basilar-membrane motion inferred by G. Zweig.</b>                                 | <b>33</b> |

## A. Supplementary Data (Figs. S1-S4)

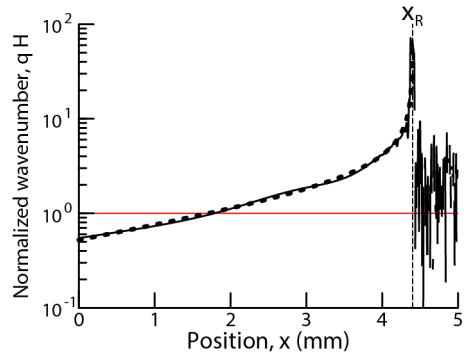

**Fig. S1. The condition for 1D-hydrodynamics breaks down over most of the distance traveled by the wave.** Longitudinal profile of the product of the wavenumber,  $q$ , by the height,  $H$ , of the compartments in the box model of the cochlea. The wavenumber was defined as  $q = -\partial_x \theta$ , where  $\theta(x)$  is the phase in radians of the oscillators' response to a 6.6 kHz stimulus at a sound-pressure level of 10 dB. The red horizontal line and the black vertical dashed line mark the condition  $qH = 1$  and the resonant place,  $x_R$ , respectively. The WKB approximation to the normalized wavenumber profile is shown as a thick dashed line. The condition for 1D-hydrodynamics is  $qH \ll 1$ . Same model, parameters (Table S1) and methodology (Table S2) as in Figure 2 in Main Text.

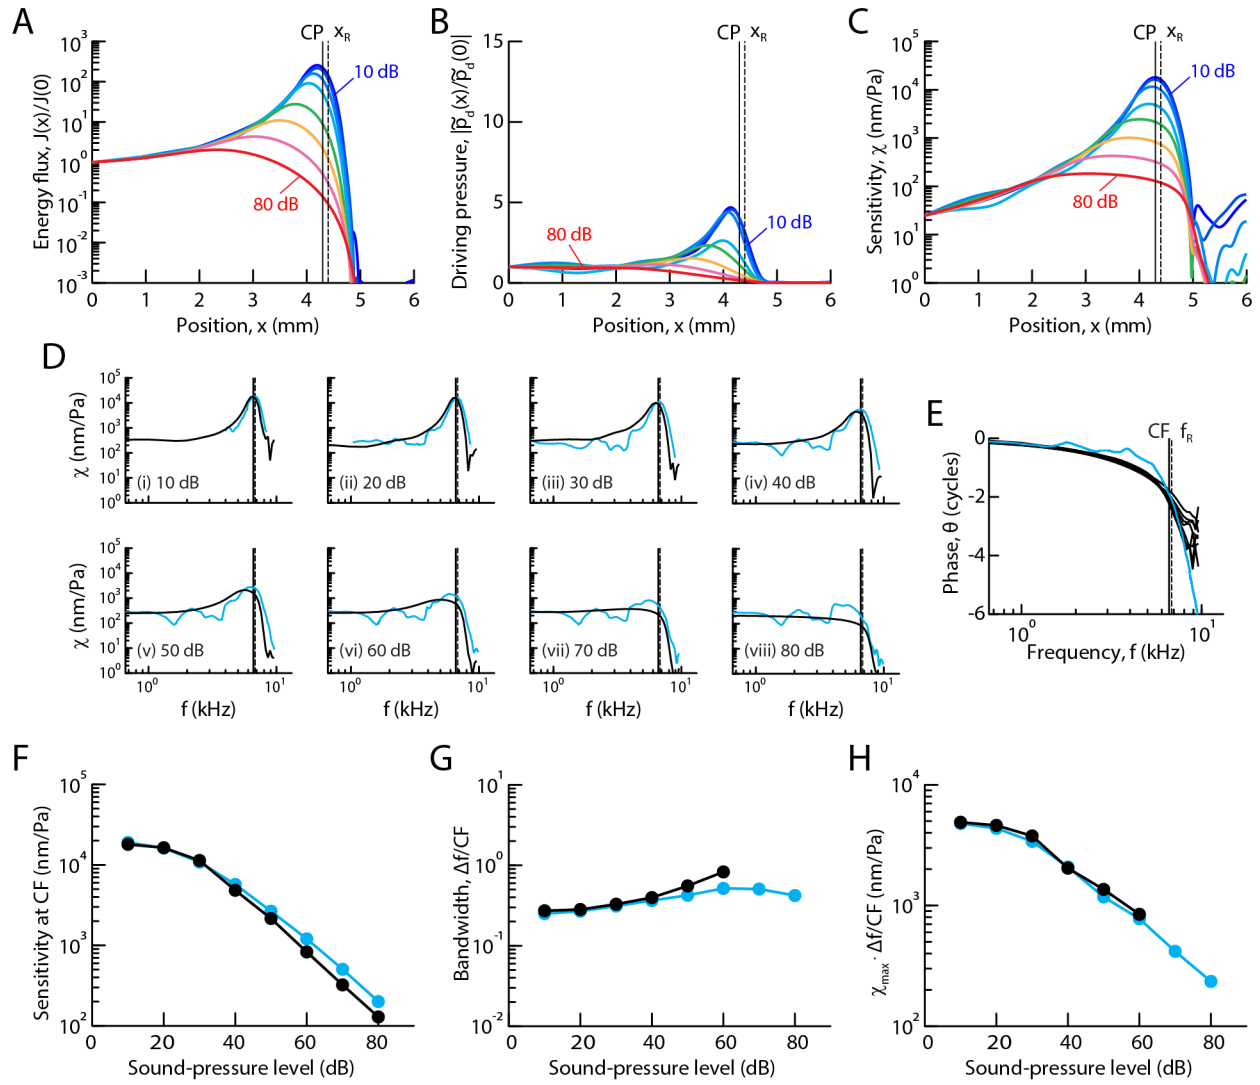

**Fig. S2. 1D effective description of the cochlea with mechanical coupling and energy pumping.** (A-C) Longitudinal profiles, respectively, of time-averaged energy flux,  $J(x)/J(0)$ , of driving pressure,  $|\tilde{p}_d(x)/\tilde{p}_d(0)|$ , and of sensitivity,  $\chi(x)$ , for a pure-tone stimulus of frequency  $f = 6.6$  kHz and at sound-pressure levels increasing from 10 dB (blue) to 80 dB (red) in 10 dB increments. The characteristic place,  $CP = 4.30$  mm, of maximal sensitivity at low sound-pressure level and the place of oscillator resonance,  $x_R = 4.40$  mm, with the stimulus are marked by vertical solid and dashed lines, respectively. (D) Comparison of frequency-tuning curves of sensitivity in the model (black) and in experiments (cyan) at a fixed position,  $x = CP(f = 6.6 \text{ kHz})$  and with sound-pressure levels increasing from 10 dB (i) to 80 dB (vi) in 10 dB increments. The characteristic frequency,  $CF = 6.6$  kHz, and the resonant frequency,  $f_R = 7.3$  kHz, of the oscillator at the position of measurement are indicated by vertical solid and dashed lines, respectively. (E) Phase of the response, relative to that at the base ( $x = 0$ ), as a function of frequency for the data shown in (D). (F-H) Level functions, respectively, of sensitivity at CF, normalized bandwidth,  $\Delta f/CF$ , and gain-bandwidth product,  $\chi_{\max} \cdot \Delta f/CF$ , for the tuning curves shown in (D), in which  $\chi_{\max}$  is the peak sensitivity. In (D-H), the results of the model (black) are confronted to experimental measurements (cyan) from [1]. Parameter values in Table S1 and methodology in Table S2.

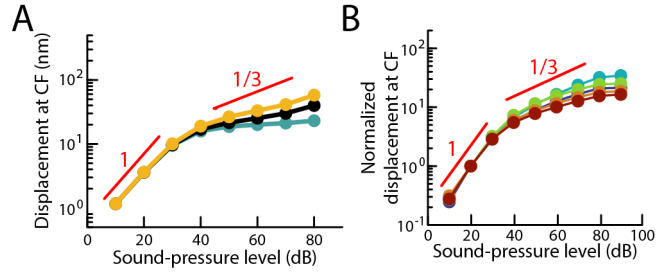

**Fig. S3. Variability of compressive nonlinearity in modeled and experimental level functions.** (A) Amplitude of the response at the characteristic frequency (CF) as a function of the sound-pressure level in the model for three values of parameter  $\beta_i$ :  $-8 \text{ nm}^{-2} \text{ s}^{-1}$  (orange),  $-4 \text{ nm}^{-2} \text{ s}^{-1}$  (black) and  $-2 \text{ nm}^{-2} \text{ s}^{-1}$  (green). Other parameters:  $\alpha = 19,500 \text{ Pa s m}^{-1}$  (here the same at all positions),  $\beta = \beta_r = 6 \text{ nm}^{-2} \text{ s}^{-1}$ ,  $\bar{\kappa}_r = 106 \text{ } \mu\text{m}^2 \text{ s}^{-1}$ ,  $\bar{\kappa}_i = -21 \text{ } \mu\text{m}^2 \text{ s}^{-1}$ ,  $\phi = \pi/2 - 0.35 \text{ rad}$ , and  $G_{\text{ME}} = 141$ . The model was solved with 2D hydrodynamics. (B) Amplitude of the basilar-membrane response at the characteristic frequency (CF), here CF = 9 kHz, as a function of the sound-pressure level in experiments from six representative mouse cochleae within an ensemble of 15. Each response was normalized by that at 20 dB. Power-law fits to the level functions for sound-pressure levels larger than 40 dB led to power-law exponents of 0.22 (yellow), 0.18 (black) and 0.06 (green) for the model (A) and an ensemble average of  $0.25 \pm 0.06$  (mean  $\pm$  SD;  $n = 15$ ) for the experiments (B). Experimental data from [2]. Frequency-tuning curves were obtained, at each sound-pressure level, from responses to pure-tone stimuli of varying frequencies.

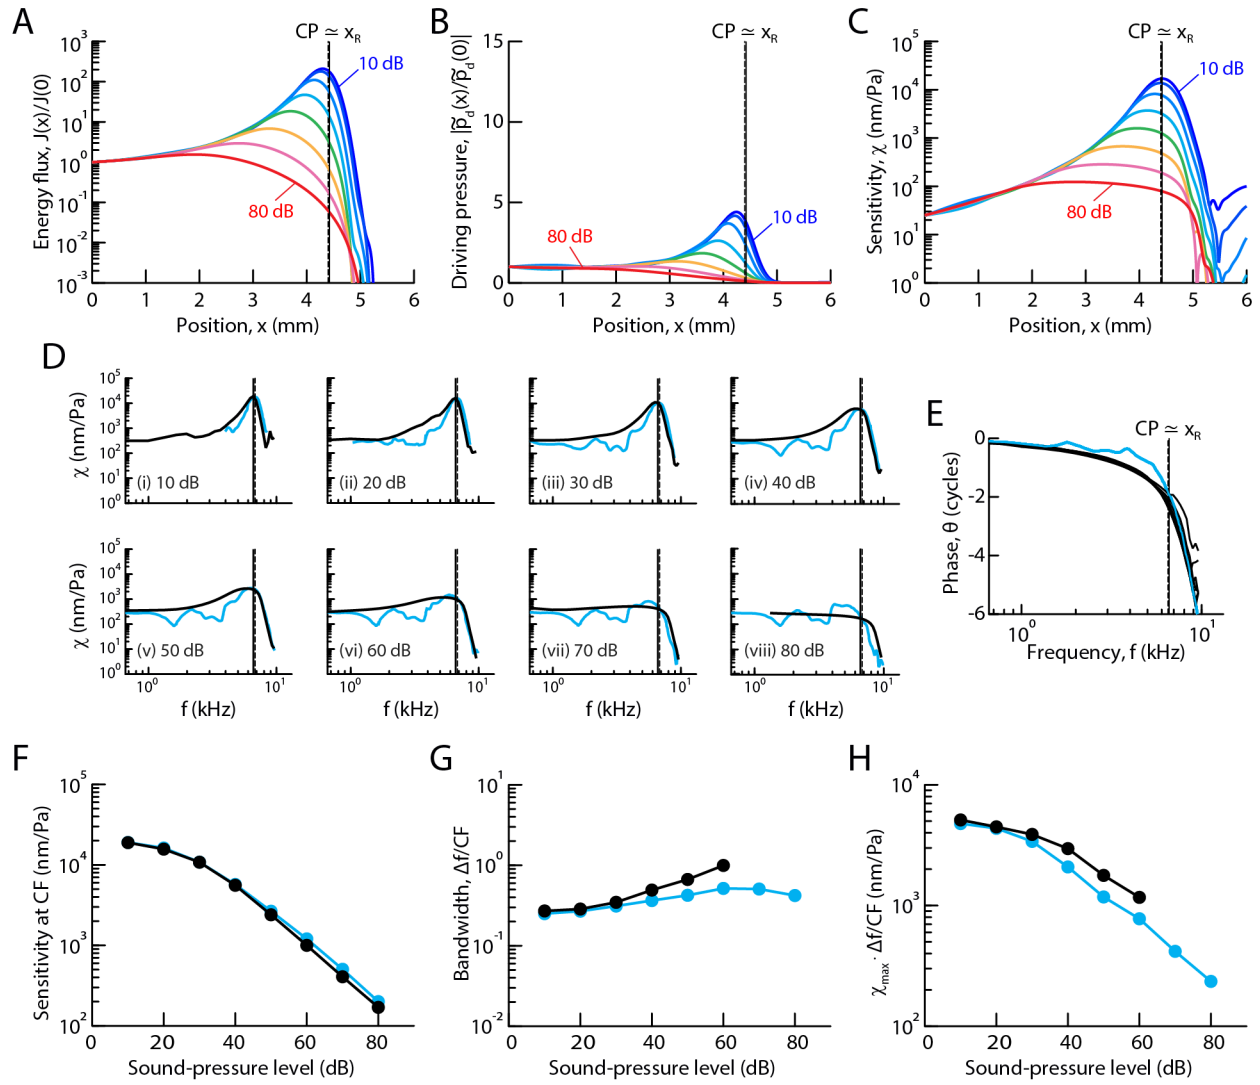

**Fig. S4. 1D effective description of the cochlea with no mechanical coupling, the oscillators detuned from criticality and energy pumping.** (A-C) Longitudinal profiles, respectively, of time-averaged energy flux,  $J(x)/J(0)$ , of driving pressure,  $|\tilde{p}_d(x)/\tilde{p}_d(0)|$ , and of sensitivity,  $\chi(x)$ , for a pure-tone stimulus of frequency  $f = 6.6$  kHz and at sound-pressure levels increasing from 10 dB (blue) to 80 dB (red) in 10 dB increments. The characteristic place, CP, of maximal sensitivity at low sound-pressure level and the place of oscillator resonance,  $x_R = 4.40$  mm, with the stimulus are nearly equal and marked by vertical solid and dashed lines, respectively. (D) Comparison of frequency-tuning curves of sensitivity in the model (black) and in experiments (cyan) at a fixed position,  $x = CP(f = 6.6$  kHz) and with sound-pressure levels increasing from 10 dB (i) to 80 dB (vi) in 10 dB increments. The characteristic frequency,  $CF = 6.6$  kHz, and the resonant frequency,  $f_R$ , of the oscillator at the position of measurement are nearly equal and indicated by vertical solid and dashed lines, respectively. (E) Phase of the response, relative to that at the base ( $x = 0$ ), as a function of frequency for the data shown in (D). (F-H) Level functions, respectively, of sensitivity at CF, normalized bandwidth,  $\Delta f/CF$ , and gain-bandwidth product,  $\chi_{max} \cdot \Delta f/CF$ , for the tuning curves shown in (D), in which  $\chi_{max}$  is the peak sensitivity. In (D-H), the results of the model (black) are confronted to experimental measurements (cyan) from [1]. Parameter values in Table S1 and methodology in Table S2.

## B. Definition and generic properties of a critical oscillator.

The generic properties of active dynamical systems near a Hopf bifurcation have been extensively discussed in the literature (e.g. [3–10]). We review here those that are essential to our work. Specifically, we define the concept of a critical oscillator, explicit the power laws that emerge in response to sinusoidal stimuli, emphasize the inverse relation between the oscillator's maximal sensitivity and the sharpness of its frequency tuning, how this relation relates to the phenomenon of "critical slowing down", and describe energy transfer between the oscillator and the environment.

A Hopf bifurcation represents an oscillatory instability upon a continuous variation of an external control parameter,  $C$ : at a critical value,  $C = C_c$ , of the control parameter, the systems undergoes an abrupt transition between a quiescent state and a dynamic state of spontaneous oscillations at a natural frequency,  $\omega_R$  [3, 4]. The system is said to be "critical" when it operates precisely at the bifurcation point, corresponding to  $\varepsilon = C - C_c = 0$ . A system operating near a Hopf bifurcation acquires generic properties that do not depend on the detailed mechanism that underlies the oscillatory instability. Specifically, the dynamics of the system can be described at steady state with only two degrees of freedom. Within the framework of our box model of the cochlea, two variables—the transverse motion of the basilar membrane,  $h$ , that is measured in experiments and an hidden variable,  $h_a$ , representing active force feedback on the basilar membrane—account for the local operation of the cochlear partition near a Hopf bifurcation. Proximity to the bifurcation dictates that the complex variable,  $z = h + ih_a$ , obeys the normal form:

$$\dot{z} \simeq (\varepsilon + i\omega_R)z - \beta|z|^2z + e^{-i\phi}\frac{F(t)}{\alpha}, \quad (\text{S1})$$

where  $\beta = \beta_r + i\beta_i$  is a complex number that sets the strength of the cubic nonlinear term with  $\beta_r > 0$  to ensure stability,  $F$  represents an external force<sup>1</sup>,  $\alpha$  is a parameter with units of a friction coefficient, and  $\phi$  is a phase parameter<sup>2</sup>. The normal form is an expansion in powers of  $z$  in which the dominant nonlinear term is cubic; there is no quadratic term. It is also invariant under the phase shift  $z \rightarrow ze^{i\varphi}$ , where  $\varphi$  is an arbitrary but constant phase. Phase invariance is not intrinsic to the original system, but emerges in the vicinity of a Hopf bifurcation.

**1. Response to a sinusoidal stimulus near a Hopf bifurcation—critical slowing down.** We study here the behavior of the normal form (Eq. (S1)) in the case of a sinusoidal stimulus,  $F(t) = \tilde{F}e^{i\omega t}$ ,

<sup>1</sup>There are generally nonlinear corrections to the driving stimulus in Eq. (S1), we kept only the linear term, implying that the drive is small enough.

<sup>2</sup>The phase parameter  $\phi$  is set by the change of variables that brings the dynamics of the system into normal form; see Appendix A in [8] for an illustrative example.

where the Fourier amplitude  $\tilde{F}$  sets the stimulus level and  $\omega$  is the angular frequency of the stimulus. We assume that the system operates on the stable side of the bifurcation, corresponding to  $\varepsilon \leq 0$ . For simplicity, we also assume that  $\beta$  is real ( $\beta_i = 0$ ). The amplitude  $\tilde{z}$  of the phase-locked response  $z(t) \simeq \tilde{z} e^{i(\omega t - \phi)}$  obeys

$$\tilde{F} = A_{zF} \tilde{z} + B |\tilde{z}|^2 \tilde{z}, \quad (\text{S2})$$

where  $B = \alpha\beta$  and  $A_{zF} = \alpha(-\varepsilon + i(\omega - \omega_R))$  is a complex modulus that characterizes the linear response. The sensitivity

$$\chi = \frac{|\tilde{z}|}{|\tilde{F}|} \quad (\text{S3})$$

peaks when the oscillator is driven at its natural frequency

$$\max(\chi) = \chi(\omega = \omega_R). \quad (\text{S4})$$

This is the signature of the resonant behavior of a system operating close to a Hopf bifurcation<sup>3</sup>. In the limit of small stimuli, the maximal sensitivity exhibits a linear regime

$$\lim_{|\tilde{F}| \rightarrow 0} \max(\chi) = \frac{1}{|A_{zF}(\omega = \omega_R)|} = \frac{1}{\alpha|\varepsilon|}. \quad (\text{S5})$$

At the critical point ( $\varepsilon = 0$ ), the system acquires a remarkable property: its sensitivity to vanishing stimuli diverges<sup>4</sup>. The amplitude of the response,  $|\tilde{z}|$ , is then under the control of the cubic term in the normal form and its relation to the stimulus amplitude displays a compressive nonlinearity given by a power law of exponent 1/3 (Fig. S5.A) :

$$|\tilde{z}| \simeq \frac{1}{(\alpha\beta_r)^{1/3}} |\tilde{F}|^{1/3}, \quad (\text{S6})$$

which leads to a maximal sensitivity that increases for decreasing stimulus levels according to a power law of exponent  $-2/3$  (Fig. S5.B):

$$\max(\chi) \simeq \frac{1}{(\alpha\beta_r)^{1/3}} |\tilde{F}|^{-2/3}. \quad (\text{S7})$$

Away from resonance ( $\omega \neq \omega_R$ ), the linear term in the normal form (Eq. (S1)) reasserts itself, leading to a linear regime of responsiveness for stimulus levels,  $|\tilde{F}| \leq \alpha|\omega - \omega_R|^{3/2}/\beta_r^{1/2}$ , that are low

<sup>3</sup>This is why we denote the natural frequency by  $\omega_R$ : the oscillator resonates in response to small sinusoidal stimuli at this frequency, hence the subscript  $R$ .

<sup>4</sup>This is a signature of the oscillator's activity. Indeed, although inertia and elasticity may cancel each other in a passive system driven at an appropriate frequency, there must be energy consumption to also compensate for the frictional contribution to the linear response at finite frequency.

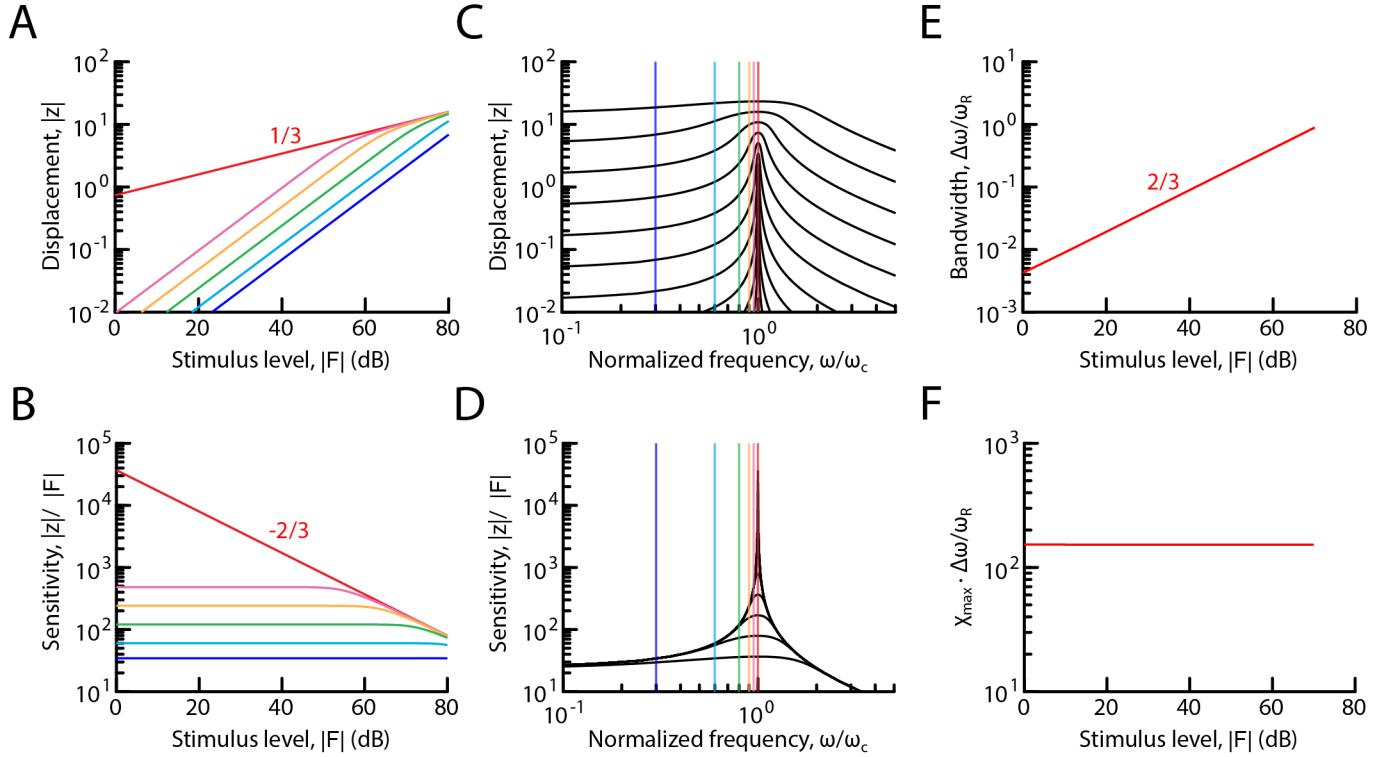

**Fig. S5.** Response of a critical oscillator to a periodic stimulus of level  $|\tilde{F}|$ , and angular frequency  $\omega$ , as described by Eq. (S2). **(A):** Modulus of the oscillator's response,  $|\tilde{z}|$ , as a function of stimulus level,  $|\tilde{F}|$ , at six fixed stimulus frequencies:  $\omega = 0.3\omega_R$  (blue),  $\omega = 0.6\omega_R$  (cyan),  $\omega = 0.8\omega_R$  (green),  $\omega = 0.9\omega_R$  (yellow),  $\omega = 0.95\omega_R$  (pink), and  $\omega = \omega_R$  (red). At the natural frequency  $\omega = \omega_R$ , the response shows a power-law behavior of exponent  $1/3$ . **(B):** Sensitivity,  $|\tilde{z}|/|\tilde{F}|$ , as a function of stimulus level,  $|\tilde{F}|$ , at the fixed stimulus frequencies  $\omega$  (color coded as in Panel A). At the natural frequency  $\omega = \omega_R$ , the sensitivity shows a power-law of exponent  $-2/3$ . **(C):** Modulus of the oscillator's response,  $|\tilde{z}|$ , as a function of normalized frequency,  $\omega/\omega_R$ . Each curve corresponds to a stimulus level,  $|\tilde{F}|$ , increasing from 0 dB (lowest displacement) to 100 dB (highest displacement) in 10 dB increments. **(D):** Tuning curve of sensitivity,  $|\tilde{z}|/|\tilde{F}|$ , as a function of normalized frequency,  $\omega/\omega_R$ . Each curve corresponds to a stimulus level,  $|\tilde{F}|$ , increasing from 0 dB (highest sensitivity) to 100 dB (lowest sensitivity) in 10 dB increments. As the stimulus gets stronger, the sensitivity at the peak of the tuning curve decreases and the peak broadens. **(E):** Bandwidth  $\Delta\omega$  of the peaks in D as a function of stimulus level. The bandwidth of the peak in D increases with stimulus level,  $|\tilde{F}|$ , following a power law of exponent  $2/3$ . **(F):** Gain-bandwidth product,  $\max(\chi) \cdot \Delta\omega$ , of the peaks in D as a function of stimulus level,  $|\tilde{F}|$ . The inverse relation between the maximum sensitivity  $\max(\chi)$  and the bandwidth gives a gain-bandwidth product that does not depend on the stimulus level. The parameters of Eq. (S2) are chosen to get a response of 1 nm at 0 dB and at the angular frequency  $\omega = \omega_R$ :  $\varepsilon = 0$  Hz,  $\omega_R = 2\pi \cdot 6.6$  kHz,  $\beta_r = 2 \cdot 10^{19} \text{ m}^{-2} \text{ s}^{-1}$ ,  $\beta_i = 0 \text{ m}^{-2} \text{ s}^{-1}$ ,  $\phi = \pi/2$ , and  $\alpha = 10^3 \text{ N s m}^{-1}$ . Reference value for the stimulus in dB,  $|\tilde{F}|_{\text{ref}} = 20 \text{ } \mu\text{N}$ . Figure adapted from [11].

enough (Fig. S5.A and B). As a result, the response is tuned (Fig. S5.C and D), with a bandwidth,  
 $\Delta\omega = |\omega - \omega_R|$  that increases with level (Fig. S5.E) as:

$$\Delta\omega \propto \frac{\beta_r^{1/3}}{\alpha^{2/3}} |\tilde{F}|^{2/3}. \quad (\text{S8})$$

Because the bandwidth is inversely related to the maximal sensitivity, the gain-bandwidth product,

$$\max(\chi) \cdot \Delta\omega \propto 1/\alpha, \quad (\text{S9})$$

is a constant: it does not depend on the stimulus level (Fig. S5.F)<sup>5</sup>. Note that other resonators, like the harmonic and van der Pol oscillators, obey the same constraint.

A critical oscillator thus responds to faint stimuli with both high sensitivity and sharp frequency selectivity, which are attractive features for hearing. There is, however, a price to pay: the weaker the stimulus, the slower the rise to a steady-state response. This is because, as for other resonant systems, the response time,  $\tau$ , in the time domain is inversely related to the bandwidth of frequency tuning and thus diverges at vanishing stimulus amplitudes:

$$\tau \propto \frac{1}{\Delta\omega} \propto \frac{\alpha^{2/3}}{\beta_r^{1/3}} \frac{1}{|\tilde{F}|^{2/3}} \xrightarrow{|\tilde{F}| \rightarrow 0} +\infty \quad (\text{S10})$$

This property is analogous to a phenomenon called "critical slowing down" for thermodynamic phase transitions and is a defining feature of criticality. Slow responsiveness is thus a fundamental property associated to the high sensitivity of a critical oscillator to weak stimuli.

**2. Linear response and energy pumping.** In this subsection, we study the power transfer between the stimulus and an oscillator operating near a Hopf bifurcation in the linear regime of responsiveness. Ignoring the nonlinear term in the normal form ( $\beta = 0$  in Eq. (S1)), the equation of motion obeys:

$$\dot{z} = (\varepsilon + i\omega_R)z + e^{-i\phi} \frac{F(t)}{\alpha}. \quad (\text{S11})$$

This equation can be written as a set of two coupled first-order equations for the real part,  $h$ , and the imaginary part,  $h_a$ , of the complex variable  $z$ :

$$\dot{h} = \varepsilon h - \omega_R h_a + \cos \phi \frac{F}{\alpha}, \quad (\text{S12})$$

$$\dot{h}_a = \omega_R h + \varepsilon h_a - \sin \phi \frac{F}{\alpha}. \quad (\text{S13})$$

<sup>5</sup> When the bandwidth is measured 10 dB below the peak sensitivity, the numerical prefactor in Eqs. (S8–S9) is about  $\sqrt{10}$ .

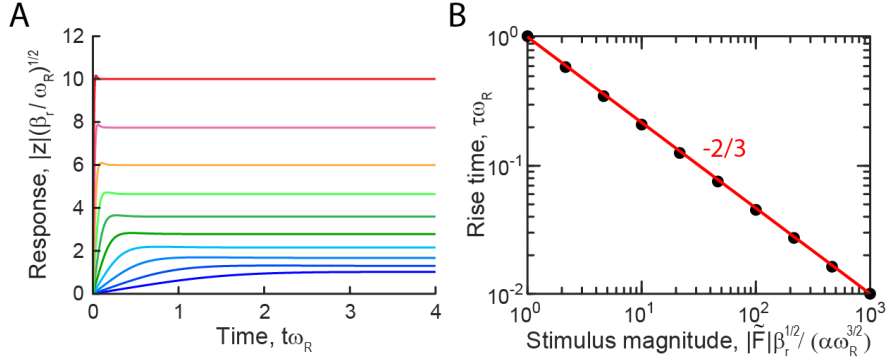

**Fig. S6.** Rise time of a critical oscillator to a steady-state response. **(A)** Response,  $|z(t)|$ , of a critical oscillator to a sinusoidal stimulus  $F(t) = \tilde{F}e^{i\omega_R t}$  at the natural frequency,  $\omega_R$ , of the oscillator as a function of time,  $t$ , for a stimulus magnitude,  $|\tilde{F}|$ , increasing by a thousandfold from 1 (blue) to  $10^3$  (red) in equal logarithmic increments. **(B)** Rise time at 95% of the steady-state response,  $\tau$ , as a function of the stimulus magnitude. The red lines marks a power law of exponent  $2/3$ . Response, stimulus and time have been normalized, respectively, by a characteristic length, force and time in the normal form. Parameter values:  $\omega_R = 1$ ,  $\beta_r = 1$ , and  $\alpha = 1$ .

Assuming that  $h$  is the observable, we can combine the two equations to eliminate  $h_a$  and get a single equation relating  $h$ ,  $F$  and their time derivatives:

$$\ddot{h} - 2\varepsilon\dot{h} + (\omega_R^2 + \varepsilon^2)h = \frac{\omega_R}{\alpha} \left[ \left( \sin \phi - \frac{\varepsilon}{\omega_R} \cos \phi \right) F + \cos \phi \frac{\dot{F}}{\omega_R} \right]. \quad (\text{S14})$$

We recognize in Eq. (S14) the equation of motion of an effective harmonic oscillator driven by a linear combination of  $F$  and  $\dot{F}$ , with an effective mass  $m_{\text{eff}} = \alpha/\omega_R$ , damping coefficient  $\xi_{\text{eff}} = -2\alpha\varepsilon/\omega_R$ , and stiffness  $k_{\text{eff}} = \alpha(\omega_R^2 + \varepsilon^2)/\omega_R$ . Importantly, because these parameters are effective, they are not directly related to the actual mass, damping coefficient, and stiffness of the basilar membrane.

Because Eq. (S14) is linear, a periodic stimulus at a frequency  $\omega$ ,  $F(t) = \tilde{F}e^{i\omega t}$ , evokes a response at the frequency of the stimulus,  $h(t) = \tilde{h}e^{i\omega t}$ . The linear response is then characterized by the frequency-dependent complex modulus,  $\mathcal{A}(\omega) = \tilde{F}/\tilde{h}$ . From Eq. (S14), the complex modulus is given by

$$\mathcal{A}(\omega) = \frac{k_{\text{eff}} - m_{\text{eff}}\omega^2 + i\omega\xi_{\text{eff}}}{\left( \sin \phi - \frac{\varepsilon}{\omega_R} \cos \phi \right) + i\frac{\omega}{\omega_R} \cos \phi}, \quad (\text{S15})$$

where we have used the parameters of the effective harmonic oscillator for simplicity. The power transfer,  $\mathcal{P}$ , from the stimulus to the oscillator is given by the time-averaged product of the stimulus,  $F$ , and the velocity of the conjugated variable,  $v = \dot{h}$ ,

$$\mathcal{P} = \int_0^T \frac{dt}{T} F(t) \cdot v(t) = 2\text{Re}[\tilde{F} \cdot (-i\omega\tilde{h}^*)] = 2\omega|\tilde{h}|^2\text{Im}[\mathcal{A}]. \quad (\text{S16})$$

In a passive system, the power performed by the stimulus must balance the power dissipated by the system, which is always negative because dissipation sucks energy out of the system; the power  $\mathcal{P}$  in

117 this case must thus be positive. In return, energy dissipation corresponds here to  $\text{Im}[\mathcal{A}] > 0$ . This  
 118 can be checked in the case of a passive harmonic oscillator, corresponding to  $\phi = \pi/2$  and  $\xi_{\text{eff}} > 0$   
 119 ( $\varepsilon < 0$ ) in Eq. (S14): energy dissipation is associated with  $\text{Im}[\mathcal{A}] > 0$ . An active system can instead  
 120 inject energy into its environment, corresponding to  $\text{Im}[\mathcal{A}] < 0$ .

121 In the case of a critical oscillator ( $\varepsilon = 0$ ), the complex modulus  $\mathcal{A} = A_r + iA_i$  is given by

$$\mathcal{A} = \alpha(\omega_R \sin(\phi) - i\omega \cos(\phi)) \frac{\omega_R^2 - \omega^2}{\omega_R^2 \sin^2(\phi) + \omega^2 \cos^2(\phi)}, \quad (\text{S17})$$

122 with real and imaginary parts:

$$A_r(\omega) = \alpha \sin(\phi) \frac{\omega_R(\omega_R^2 - \omega^2)}{\omega_R^2 \sin^2(\phi) + \omega^2 \cos^2(\phi)}, \quad (\text{S18})$$

$$A_i(\omega) = -\alpha \cos(\phi) \frac{\omega(\omega_R^2 - \omega^2)}{\omega_R^2 \sin^2(\phi) + \omega^2 \cos^2(\phi)}. \quad (\text{S19})$$

123 The expression of  $A_i$  reveals that the phase parameter  $\phi$  in the stimulus driving the oscillator plays  
 124 an important role in determining power transfer between a critical oscillator and its environment.  
 125 The range of values for  $\phi$  is limited to  $\phi \in [0, \pi/2]$  to ensure positive stiffness at low frequencies  
 126 and positive friction at high frequencies, corresponding to  $\lim_{\omega \rightarrow 0} A_r > 0$  and  $\lim_{\omega \rightarrow \infty} A_i > 0$ ,  
 127 respectively.

128 Let us first consider the general case where  $\phi \neq \pi/2$ . When the oscillator is driven below its  
 129 natural frequency  $\omega < \omega_R$ , power is transferred from the critical oscillator to the environment: the  
 130 stimulus sucks energy from the oscillator to slow it down; in other words, the oscillator pumps  
 131 energy into the stimulus. Instead, when it is driven above its characteristic frequency  $\omega > \omega_R$ , power  
 132 is transferred from the stimulus to the oscillator, as in the case of a passive system: the stimulus  
 133 injects energy into the oscillator to make it oscillate faster (Fig. S7.A). For a stimulus at the natural  
 134 frequency,  $\omega = \omega_R$ , both  $A_r$  and  $A_i$  are null. Remarkably enough, in the singular case for which  
 135  $\phi = \frac{\pi}{2}$ ,  $A_i$  is null at all driving frequencies (Fig. S7.B): there is no net power injection nor dissipation  
 136 by the critical oscillator. The oscillator is still active because dissipation has been canceled (here at  
 137 all frequencies, not just at  $\omega = \omega_R$ ). Note that in this case the effective harmonic oscillator that  
 138 describes the linear response of a critical oscillator is simply driven by  $F$ : the prefactor of  $\dot{F}$  is null.  
 139 In return, we see that the ability of a critical oscillator to pump energy into the stimulus at  $\omega < \omega_R$   
 140 is equivalent to representing its linear behavior as that of an harmonic oscillator driven by a linear  
 141 combination of  $F$  and its time derivative (Eq. (S14)).

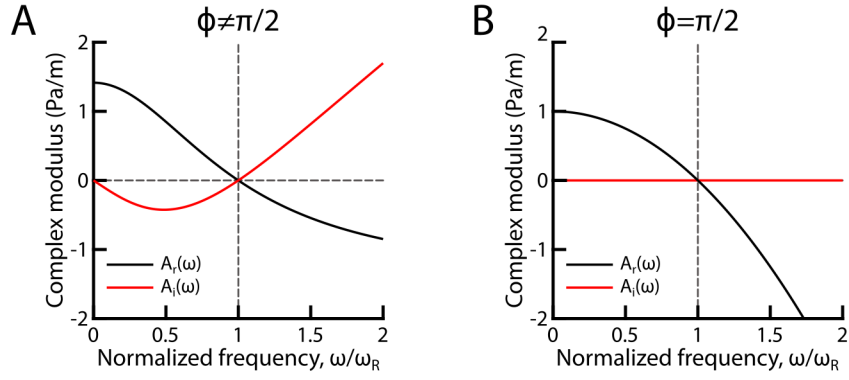

**Fig. S7.** The phase parameter  $\phi$  controls the power transfer between a Hopf oscillator and its environment. Real part  $A_r$  (blue) and imaginary part  $A_i$  (red) of the complex modulus  $\mathcal{A}$  of a Hopf oscillator (Eq. (S15)). **(A):** Critical oscillator ( $\varepsilon = 0$ ) with  $\phi = \pi/4$ . **(B):** Critical oscillator ( $\varepsilon = 0$ ) with  $\phi = \pi/2$ . Other parameters:  $\alpha = 1$ , and  $\omega_R = 2\pi$ .

Note that the phase parameter  $\phi$  changes the elastic response of the critical oscillator: the complex modulus at  $\omega = 0$  can be interpreted as the oscillator's stiffness  $k_{\text{eff}} = \mathcal{A}(0) = A_r(0) = \frac{\alpha\omega_R}{\sin(\phi)}$ . As the phase parameter decreases from  $\phi = \pi/2$  to  $\phi = 0$ , the elastic response of the critical oscillator decreases, or equivalently, the critical oscillator gets stiffer. If a Hopf oscillator is detuned from criticality ( $\varepsilon \neq 0$ ), the real and imaginary parts of the linear response do not cancel precisely at the same frequency. In that case, there is no frequency at which  $\mathcal{A} = 0$ . The oscillator can still pump energy into its environment but over a smaller range of frequencies.

## C. Box model of the cochlea based on critical oscillators

The cochlea is described by a rectangular box of length  $L$  and height  $2H$  (see Fig. 1 in Main text). Longitudinal and transverse coordinates are called  $x$  and  $y$ , respectively. We consider that all fields are uniform along the third dimension; the model is thus two-dimensional. The box is divided into two compartments by a line at  $y = 0$  that represents the cochlear partition. The boundary at  $x = 0$  is an open end; sound evokes a pressure stimulus that is injected at this boundary in the upper compartment. The upper and lower boundaries of the box, located at  $y = H$  and  $y = -H$ , respectively, are rigid. Additionally, a hole at  $x = L$  connects the two compartments, modeling the helicotrema in the cochlea.

**1. Description of the partition as a chain of critical oscillators.** The basilar-membrane that supports the cochlear partition is described in the model as a chain of tonotopically-distributed critical oscillators. Each oscillator obeys an equation of motion given by the normal form (Eq. (S1)), with

161 added mechanical coupling between the nearest neighbors:

$$\partial_t z = (\varepsilon + i\omega_R(x))z - \beta|z|^2 z + \kappa(x)\partial_x^2 z + e^{-i\phi} \frac{p_d}{\alpha(x)}. \quad (\text{S20})$$

162 The real part,  $h = \text{Re}[z]$ , of the complex variable  $z(x, t)$  describes the transverse displacement of  
 163 the basilar membrane. The control parameter,  $\varepsilon = 0$ , ensures that the oscillators are all critical.  
 164 The natural frequency of each oscillator,  $\omega_R(x) = \omega_0 \exp(-x/d)$ , decreases exponentially along the  
 165 longitudinal,  $x$ -axis of the box to account for the tonotopic map of the cochlea, with a characteristic  
 166 length  $d$  and a natural frequency  $f_0 = \omega_0/(2\pi)$  at the base. Parameter  $\beta = \beta_r + i\beta_i$ , which sets the  
 167 strength of the cubic nonlinearity, has real and imaginary parts,  $\beta_r$  and  $\beta_i$ , respectively. Parameter  
 168  $\alpha(x)$  is real and sets the response magnitude at low frequencies (i.e. stiffness) and  $p_d(x, t)$  is the  
 169 driving pressure at position  $x$  and time  $t$  (see Eq. (S32) below). We assume that  $\alpha(x) = \bar{\alpha}\omega_R(x)$ .  
 170 The third term on the right-hand side of Eq. (S20) accounts for mechanical coupling between  
 171 the oscillators [12] with a coupling strength  $\kappa(x) = \kappa_r(x) + i\kappa_i(x)$ . Its real and imaginary parts,  
 172  $\kappa_r(x) = \bar{\kappa}_r\omega_R(x)$  and  $\kappa_i(x) = \bar{\kappa}_i\omega_R(x)$ <sup>6</sup>, correspond to dissipative and elastic coupling, respectively;  
 173 they both decreased with distance from the base according to the tonotopic map. Coupling introduces  
 174 second-order spatial derivatives of  $z$ , which calls for two boundary conditions; we chose:

$$\partial_x^2 z|_{x=0} = 0 \quad (\text{S21})$$

$$z|_{x=L} = 0 \quad (\text{S22})$$

175 Parameter  $\phi$  is a phase shift to the driving pressure,  $p_d$ , that arises from the change of variable to  
 176 bring the system's dynamics into normal form [8]. Finally, parameters  $\beta$  and  $\phi$  are assumed to be  
 177 independent of position  $x$ .

178 The introduction of an adjustable phase shift  $\phi$  between the driving pressure  $p_d$  and the complex  
 179 variable  $z$  is an important addition to previous cochlear models based on critical oscillators [12, 13].  
 180 In those models, the phase shift was fixed at the singular value  $\phi = \pi/2$ , for which there is no net  
 181 power transfer between the oscillators and the environment to linear order (see Fig. S7). Here, we  
 182 study instead the general case  $\phi \in [0, \pi/2]$ , for which critical oscillators generically pump energy  
 183 into their environment when they are driven below their natural frequency  $\omega_R$ .

184 **2. Box model with two-dimensional hydrodynamics.** The box is filled with an inviscid and in-  
 185 compressible fluid. A sound-evoked stimulus at  $x = 0$  changes the pressure in the upper and lower

<sup>6</sup>This choice roughly accounts for mechanical gradients along the longitudinal axis of the cochlea.

186 compartments. These changes are noted  $P^{(1)}(x, y, t)$  and  $P^{(2)}(x, y, t)$ , respectively. Pressure gradients  
 187 generate fluid motion of velocity  $\mathbf{U}^{(1)}(x, y, t)$  and  $\mathbf{U}^{(2)}(x, y, t)$ . The incompressibility condition and  
 188 the equation of fluid motion take the form:

$$\nabla \cdot \mathbf{U}^{(i)} = 0, \quad (\text{S23})$$

$$\rho \partial_t \mathbf{U}^{(i)} = -\nabla P^{(i)}, \quad (\text{S24})$$

189 for  $i = 1, 2$  and where  $\rho$  is the density of the fluid. The combination of equations (S23) and (S24)  
 190 indicates that both pressure fields obey the Laplace equation:

$$\Delta P^{(i)} = 0. \quad (\text{S25})$$

191 The hydrodynamic model with boundary conditions is shown in Fig. S8A.

192 Because the only open end is at the site of stimulus injection ( $x = 0$ ) and the boundaries at  $y = H$   
 193 and  $y = -H$  are rigid (i.e.  $U_y^{(1)}|_{y=H} = U_y^{(2)}|_{y=-H} = 0$ ), the total fluid flux in any cross-section of the  
 194 box is null, which leads to a property of anti-symmetry with respect to  $y = 0$ <sup>7</sup>, across the partition:

$$U_x^{(1)}(x, y) = -U_x^{(2)}(x, -y), \quad (\text{S26})$$

$$P^{(1)}(x, y) = -P^{(2)}(x, -y), \quad (\text{S27})$$

195 which in combination with Eq. (S24) leads to

$$U_y^{(1)}(x, y) = U_y^{(2)}(x, -y). \quad (\text{S28})$$

196 Due to this property, we can reduce the problem to the upper compartment of the box by  
 197 considering the velocity field  $\mathbf{u} = (u_x, u_y)$  and the pressure  $p$  field defined as:

$$u_x(x, y) = U_x^{(1)}(x, y) - U_x^{(2)}(x, -y) = 2U_x^{(1)}(x, y), \quad (\text{S29})$$

$$u_y(x, y) = U_y^{(1)}(x, y) + U_y^{(2)}(x, -y) = 2U_y^{(1)}(x, y), \quad (\text{S30})$$

$$p(x, y) = P^{(1)}(x, y) - P^{(2)}(x, -y) = 2P^{(1)}(x, y), \quad (\text{S31})$$

198 with  $0 \leq x \leq L$  and  $0 \leq y \leq H$ . The pressure,  $p_d$ , that drives transverse motion of the oscillators is  
 199 given by

$$p_d(x) = p(x, y = 0). \quad (\text{S32})$$

<sup>7</sup> Because sound-evoked motion of the stapes in the middle ear ought to only affect pressure in scala vestibuli, the anti-symmetry property appears to be violated at the base:  $P^{(1)}(x = 0, y) = P_b(y)$  whereas  $P^{(2)}(x = 0) = 0$ . However, fluid incompressibility dictates that pressure in the two compartments instantaneously adjust to  $P^{(1)}(x = 0, y) = P_b(y)/2$  and  $P^{(2)}(x = 0, -y) = -P_b(y)/2$ , thus restoring anti-symmetry while keeping the pressure difference  $P^{(1)}(x = 0, y) - P^{(2)}(x = 0, -y) = P_b$

200 Using Eqs. (S23-S24), the fields (S29-S31) obey:

$$\nabla \cdot \mathbf{u} = 0, \quad (\text{S33})$$

$$\rho \partial_t \mathbf{u} = -\nabla p. \quad (\text{S34})$$

201 The pressure field  $p$  is thus solution of the Laplace equation:

$$\Delta p = 0. \quad (\text{S35})$$

202 We now specify boundary conditions. The upper and lower boundaries of the box are rigid,  
 203  $U_y^{(1)}|_{y=H} = U_y^{(2)}|_{y=-H} = 0$ , and thus  $u_y|_{y=H} = 0$ . At  $y = 0$ , the transverse fluid velocity matches  
 204 the velocity of the partition  $U_y^{(1)}|_{y=0} = U_y^{(2)}|_{y=0} = -\partial_t h$  and thus  $u_y|_{y=0} = -2\partial_t h$ <sup>8</sup>. Note that, by  
 205 convention, the transverse displacement of the partition,  $h$ , is defined positive when the partition  
 206 moves toward the bottom compartment, corresponding to a positive driving pressure  $p_d = p(x, y = 0)$ .  
 207 Together with Eq. (S34), we get:

$$\partial_y p|_{y=H} = 0, \quad (\text{S36})$$

$$\partial_y p|_{y=0} = 2\rho \partial_t^2 h \quad (\text{S37})$$

208 At  $x = L$ , because the lower and upper compartments are connected, we impose:

$$p|_{x=L} = 0. \quad (\text{S38})$$

209 At  $x = 0$ , the stimulus  $P_b(y, t)$  modulates the pressure at the base of the box (see Section C4):

$$p|_{x=0} = P_b(y, t). \quad (\text{S39})$$

210 Overall, the 2D model is defined by Eqns.(S20-S22) and (S35-S39).

211 **3. Box model with one-dimensional hydrodynamics.** With 1D hydrodynamics, the pressure field  
 212  $p(x)$  obeys [13]

$$\partial_x^2 p = \frac{2\rho}{H} \partial_t^2 h. \quad (\text{S40})$$

213 The boundary conditions are

$$p(x = 0) = P_b(t) \quad (\text{S41})$$

$$p(x = L) = 0 \quad (\text{S42})$$

<sup>8</sup>The vibration magnitude of the basilar membrane that supports the cochlear partition varies within a range of 1 – 100 nm [14]. This is at least three orders of magnitude smaller than the wavelength of traveling waves ( $\sim 100 \mu\text{m}$  near the peak vibration). As a consequence, boundary conditions at the partition, positioned at  $y = -h$ , can be evaluated at  $y = 0$ . This is also why we neglected convective terms in the equations of motion for the fluid (Eq. (S24) and Eq. (S34)).

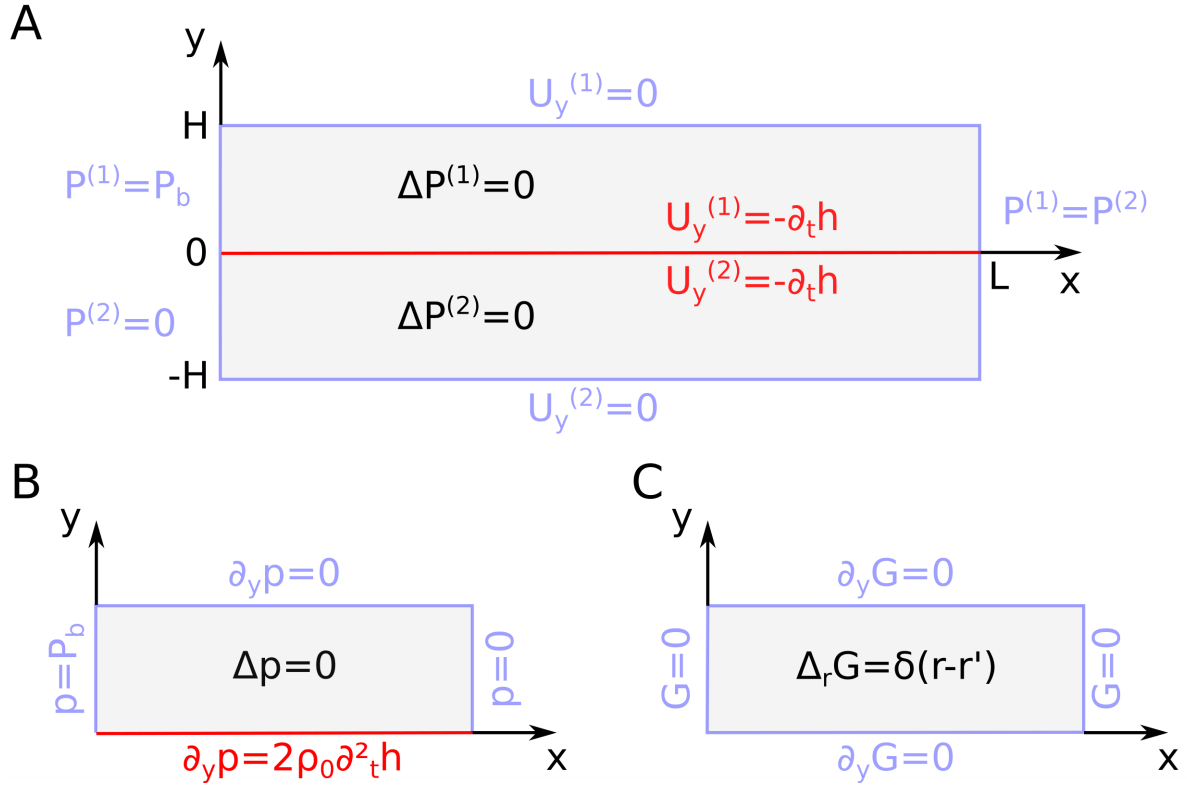

**Fig. S8.** Hydrodynamic model and boundary conditions. **(A):** Box model of the cochlea for an incompressible fluid with two dimensional fluid flows. **(B):** Equivalent model (Eqs. (S35–S39)) expressed in a single compartment for the pressure difference between the compartments as defined by Eq. S31. **(C):** Mathematical problem defining the Green function associated to the model defined in Panel B (see Section D1).

The 1D model can be obtained from the 2D model in the limit of small box height  $H$ . Overall, the 1D model is defined by Eqns.(S20-S22) and (S40-S42).

**4. Pure-tone stimulus to the box model.** The input stimulus at the base of our box model of the cochlea (Eq. (S39)) is related to the pressure,  $P_{EC}(t)$ , representing the pressure in the ear canal. We applied pure-tone stimuli of frequency  $f$  and amplitude  $P_0$ :

$$P_{EC}(t) = W(t)P_0 \sin(2\pi ft). \quad (S43)$$

The rise of the stimulus was conditioned by the function  $W(t)$ , which obeyed

$$W(t) = \begin{cases} (1 - \cos(\pi t/T_{tk}))/2 & \text{if } t < T_{tk} \\ 1 & \text{if } t \geq T_{tk} \end{cases} \quad (S44)$$

with a characteristic time,  $T_{tk} = 5/f$ , equal to five stimulus periods. The sound-pressure level is often expressed in decibels:

$$I_{dB} = 20 \log_{10}(\sqrt{\langle P_{EC}(t)^2 \rangle_t} / P_{REF}). \quad (S45)$$

222 where  $P_{\text{REF}}$  is a reference pressure set at  $= 20 \mu\text{Pa}$ , and  $\sqrt{\langle P_{\text{EC}}(t)^2 \rangle_t} = P_0/\sqrt{2}$  (see Eq. (S43)).

223 In the simple case for which pressure at the base does not vary along the  $y$ -axis (i.e. with 1D  
224 hydrodynamics), we write

$$P_b(t) = G_{\text{ME}} P_{\text{EC}}(t), \quad (\text{S46})$$

225 where  $P_{\text{EC}}(t)$  is the sound pressure in the ear canal and  $G_{\text{ME}}$ —the middle-ear gain—accounts for the  
226 increase in pressure mediated by the middle ear. In this work, we assumed that  $G_{\text{ME}}$  is a constant  
227 parameter that does not depend on sound frequency<sup>9</sup>.

228 The pressure in the fluid generally depends on the  $y$ -coordinate, which can generate a mismatch  
229 when pressure applied at the base of the box is homogeneous (Eq. (S46)). Such mismatch leads  
230 to a basal region in which pressure varies from that at the boundary to the bulk solution. At the  
231 relatively low frequencies of stimulation that we used in our work ( $f < 7.5 \text{ kHz}$ ), however, this  
232 boundary effect did not affect the oscillators' peak responses, for they were positioned way outside  
233 the region of pressure mismatch. In practice, to minimize this boundary effect, we matched the  
234 pressure at the base with the analytical solution to the model (Eqs. (S35–S39)) under the WKB  
235 approximation [17, 18] (see Section E below):

$$P_b(y, t) = \langle P_b \rangle_y \frac{q_0 H}{\sinh(q_0 H)} \cosh(q_0(H - y)), \quad (\text{S47})$$

236 where the average  $\langle P_b \rangle_y$  of  $P_b$  along the  $y$ -axis obeys

$$\langle P_b \rangle_y(t) = \frac{1}{H} \int_0^H P_b(y, t) dy = G_{\text{ME}} P_{\text{EC}}(t), \quad (\text{S48})$$

237 and the wavenumber  $q_0$  is the solution of the dispersion relation

$$q_0 H \tanh(q_0 H) = \frac{2\omega^2}{\mathcal{A}(x=0)}, \quad (\text{S49})$$

238 where the complex modulus,  $\mathcal{A}(x=0) = \tilde{p}_d/\tilde{h} \simeq \alpha\omega_0/\sin(\phi)$  (Eq. (S17) with  $\omega_0 \gg \omega$ ). In Eq. (S49),  
239 the frequency  $\omega$  corresponds to the angular frequency of a single-tone stimulus,  $\omega = 2\pi f$  (Eq. (S43)).

240 **5. Output of the model: Response of the oscillators, driving pressure and energy flux.** The  
241 response,  $h(x, t) = \text{Re}[z(x, t)]$ , of each oscillator was computed as a function of position and time for  
242 pure-tone stimuli of varying amplitude,  $P_0$ , and frequency,  $f$  (Eq. (S43)). After the response had

<sup>9</sup> Although the middle-ear gain displays band-pass properties in humans [15], it remains near a value of  $G_{\text{ME}} = 10$  (or 20dB) in chinchilla [16], which will serve as a reference animal model to confront theory to experiments.

grown to a steady-state magnitude, we estimated its Fourier component,  $\tilde{h}(x, \omega) = \int h(x, t) e^{-i\omega t} dt$  at the angular frequency,  $\omega = 2\pi f$ , of the stimulus over a time window of typically 50 cycles. We also computed the phase of each oscillators' vibration as  $\theta(x, \omega) = \arg(\tilde{h}(x, \omega)) - \arg(\tilde{h}(x = 0, \omega))$  and the wavenumber associated to the traveling wave of oscillator vibration as  $q(x, \omega) = -\partial_x \theta$ . The model also provided the pressure,  $p_d(x, t)$ , driving the oscillators as a function of position and time. We explain in Section E how the energy flux,  $J(x)$  was computed as a function of position from  $p_d(x, t)$  using the WKB approximation.

The sensitivity of the oscillator was defined as

$$\chi(x, \omega) = |\tilde{h}(x, \omega) / \tilde{P}_{EC}(\omega)|. \quad (\text{S50})$$

A frequency tuning curve is given by a plot of sensitivity  $\chi$  at a fixed position as a function of the stimulus frequency  $f$  at a fixed sound-pressure level in decibel (Eq. (S45)).

## D. Methods to solve the model

**1. Solution for the pressure field using the Green-function method.** To solve the Laplace equation for the pressure field  $p(x, y, t)$  (Eq. (S35)) with boundary conditions specified by Eqs. (S36–S39), see Fig. S8B, we followed a standard procedure based on the Green-function method [19], as done previously for other cochlear box models [20–22].

The Green function  $G(x, y, x', y')$  associated to the Laplace operator is the solution of

$$\Delta_{\mathbf{r}'} G = \delta(x - x') \delta(y - y'), \quad (\text{S51})$$

where  $\delta$  is a Dirac distribution and the Laplacian is computed with respect to the coordinates  $\mathbf{r}' = (x', y')$ . This equation holds within the box  $S_0 = [0, L] \times [0, H]$  and must satisfy boundary conditions, which will be specified below.

We can write:

$$p(\mathbf{r}) = \int_{S_0} dS' p(\mathbf{r}') \Delta_{\mathbf{r}'} G(\mathbf{r}, \mathbf{r}'), \quad (\text{S52})$$

which leads to

$$p(\mathbf{r}) = \int_{C_0} dl' p(\mathbf{r}') \mathbf{n}(\mathbf{r}') \cdot \nabla_{\mathbf{r}'} G(\mathbf{r}, \mathbf{r}') - \int_{C_0} dl' G(\mathbf{r}, \mathbf{r}') \mathbf{n}(\mathbf{r}') \cdot \nabla_{\mathbf{r}'} p(\mathbf{r}'), \quad (\text{S53})$$

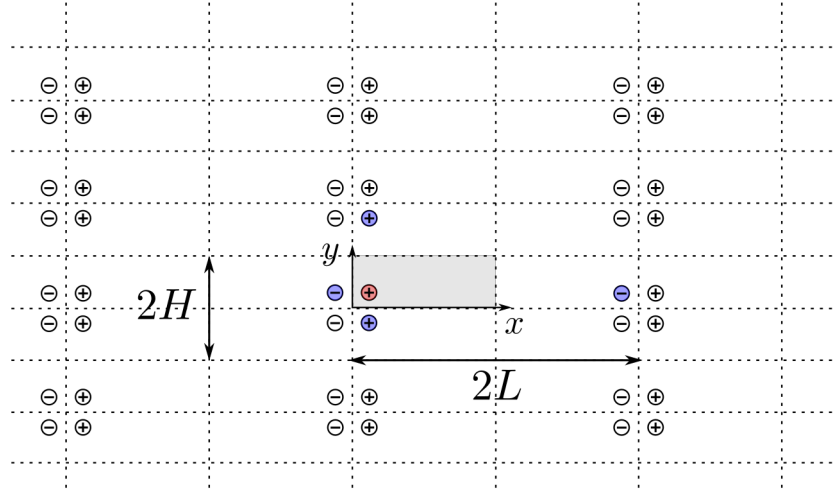

**Fig. S9.** Illustration of the method of images. A point source (red point; positive) within the equation domain (grey area) is compensated at each of the four boundary segments by additional point sources (blue points) that ensure specific boundary values for the Green function and its gradient in the normal direction to the domain contour. Additional points (black) are then added iteratively.

where we used the divergence theorem and Eq. (S35). The boundary of the box is denoted  $C_0$  and  $\mathbf{n}$  is the outward pointing unit normal at each point of  $C_0$ . Using the boundary conditions for  $p(\mathbf{r})$  (Eqs. (S36–S39)) and imposing the following boundary conditions for  $G$ :

$$G|_{x'=0} = 0, G|_{x'=L} = 0, \quad (\text{S54})$$

$$\partial_{y'} G|_{y'=0} = 0, \partial_{y'} G|_{y'=H} = 0, \quad (\text{S55})$$

we obtain

$$p(\mathbf{r}, t) = - \int_0^H dy' P_b(y', t) \partial_{x'} G(\mathbf{r}, \mathbf{r}')|_{x'=0} + 2\rho \int_0^L dx' \partial_t^2 h(x', t) G(\mathbf{r}, \mathbf{r}')|_{y'=0}, \quad (\text{S56})$$

where the first and second term on the right-hand side correspond, respectively, to the contribution of the stimulus at the base of the box ( $x = 0$ ) and that of the moving partition ( $y = 0$ ) to the pressure field within the box. Thus, the Green-function method allows to express the pressure field  $p(\mathbf{r})$  that solves the model in Fig. S8B as an integral formula that depends on the Green function  $G$  that solves the model in Fig. S8C.

The solution,  $G$ , of Eq. (S51) subject to the boundary conditions (S54–S55) is unique. To find  $G$ , we used the image method. The Green function  $G_\infty(\mathbf{r}, \mathbf{r}')$  that solves Eq. (S51) in an infinite box  $(x, y \in ] - \infty, +\infty[)$  is

$$G_\infty(\mathbf{r}, \mathbf{r}') = \frac{1}{2\pi} \log(|\mathbf{r} - \mathbf{r}'|) = \frac{1}{2\pi} \log \left( \sqrt{(x - x')^2 + (y - y')^2} \right). \quad (\text{S57})$$

276 Note that the Green function,  $G_\infty$ , can be interpreted as the electric potential that is generated by a  
 277 positive point charge at position  $\mathbf{r}$  (using dimensionless units). Using the superposition principle, the  
 278 Green function  $G$  can be derived from  $G_\infty$  by considering the distribution of point charges shown in  
 279 Figure S9; this charge distribution ensures that the boundary conditions (Eqs. (S54–S55)) for our  
 280 problem are satisfied<sup>10</sup>. We find [23]:

$$G(x, y; x', y') = \sum_{p=-\infty}^{+\infty} \sum_{q=-\infty}^{+\infty} \delta(x - p2L, y - q2H) * \mathcal{E}(x, y; x', y') * G_\infty(x, y; 0, 0), \quad (\text{S58})$$

281 with

$$\mathcal{E}(\mathbf{r}, \mathbf{r}_0) = \delta(x - x', y - y') - \delta(x + x', y - y') + \delta(x - x', y + y') - \delta(x + x', y + y'). \quad (\text{S59})$$

282 This expression can be simplified using Fourier analysis [24], leading to

$$G(x, y; x', y') = S(x; x') - \sum_{n=1}^{+\infty} T_n(x; x') \cos(k_n y) \cos(k_n y'), \quad (\text{S60})$$

283 where  $k_n = \frac{\pi}{H}n$ , and where the function  $S(x, x')$  and  $T_n(x, x')$  take the form

$$S(x; x') = \frac{1}{H} \begin{cases} -x' \left(1 - \frac{x}{L}\right) & \text{if } x \geq x' \\ -x \left(1 - \frac{x'}{L}\right) & \text{if } x < x' \end{cases}, \quad (\text{S61})$$

284 and

$$T_n(x; x') = \frac{2}{k_n H \sinh(k_n L)} \begin{cases} \sinh(k_n(L - x)) \sinh(k_n x') & \text{if } x \geq x' \\ \sinh(k_n(L - x')) \sinh(k_n x) & \text{if } x < x' \end{cases}. \quad (\text{S62})$$

285 The Green function  $G(0 \leq x \leq L, 0 \leq y \leq H, x' = L/3, y' = H/5)$  is shown in Fig. S10A.

286 The pressure driving the transverse motion of the partition,  $p_d(x, t) = p(x, y = 0, t)$  (Eq. (S32)),  
 287 can be obtained by combining Eq. (S56) and Eq. (S60), yielding the following form:

$$p_d(x, t) = - \int_0^H dy' P_b(y', t) \partial_{x'} G(\mathbf{r}, \mathbf{r}')|_{x'=0} + 2\rho \int_0^L dx' \partial_t^2 h(x', t) g(x, x'), \quad (\text{S63})$$

288 where we have introduced a reduced Green function

$$g(x, x') = G(x, y = 0; x', y' = 0) = S(x; x') - \sum_{n=1}^{+\infty} T_n(x; x'). \quad (\text{S64})$$

289 The reduced Green function  $g(x, x')$  can be interpreted as the driving-pressure profile generated by a  
 290 point-like acceleration of the partition at position  $x'$  (Fig S10B). Notably, a local acceleration of the  
 291 partition induces a driving pressure at all positions along the partition, illustrating the long-range  
 292 nature of hydrodynamic interactions.

<sup>10</sup>We use here the standard "image method": to get  $G = 0$  or  $\mathbf{n} \cdot \nabla G = 0$  at a boundary, the charge distribution must be anti-symmetric or symmetric with respect to that boundary, respectively.

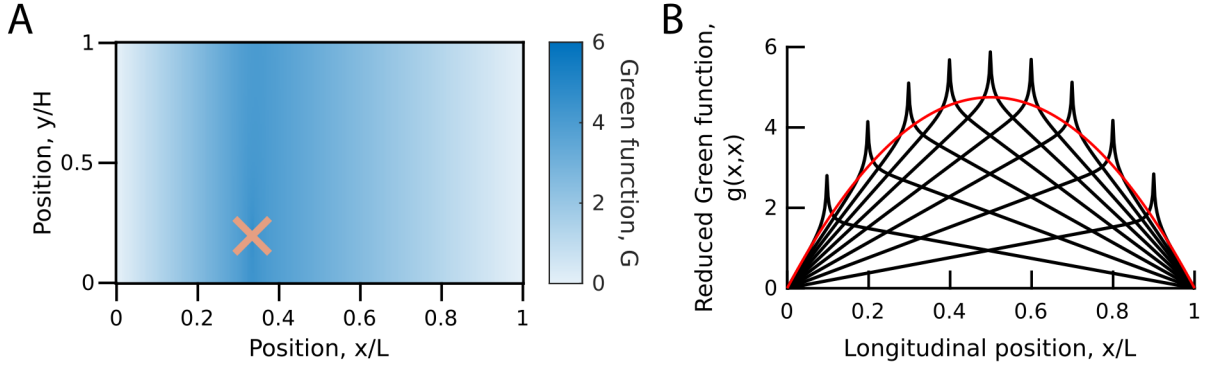

**Fig. S10.** Green function of the 2D Laplace operator with two Dirichlet boundary conditions at  $x = 0$  and  $x = L$  and two Neumann boundary conditions at  $y = 0$  and  $y = H$  with  $L/H = 19$ . **(A):** Green function,  $G(x, y; x', y')$ , as defined by Eq. (S60) with  $(x', y') = (L/3, H/5)$  (brown cross). **(B):** Magnitude of the reduced Green function,  $g(x, x') = G|_{y=y'=0}$ , as defined by Eq. (S64) for 9 values of  $x'$  regularly spaced from  $x' = L/10$  in steps of  $L/10$ . The red line indicates the maxima of  $S(x, x')$  (Eq. (S61)) which follows a parabola. Parameters:  $L = 19$  mm,  $H = 1$  mm, the sum in Eq. (S60) was cut at  $n = 100$ .

## 2. Numerical resolution of the model.

**2.a. With 2D hydrodynamics.** We solved the hydrodynamic model (Eqs. (S60-S62) and (S63-S64)) together with the model for the cochlear partition (Eq. (S20)) that is subjected to the boundary conditions given by Eqs. (S21) and (S22). The expression of the stimulus at the base  $P_b(y, t)$  is given by Eqs. (S47-S49) in Section C4. This model is solved using a finite-difference method in time domain, which we detail below.

Numerical schemes that relied on the explicit computation of  $\partial_t^2 h$  in Eq. (S63) were numerically unstable. Following the approach in Ref. [12], we circumvented this problem by using Eq. (S20) to express  $\partial_t^2 h = \partial_t^2 \text{Re}[z]$  as a function of  $z$ ,  $z^*$ ,  $p_d$  and  $\partial_t p_d$ , yielding

$$\partial_t^2 h = \mathcal{A} + \mathcal{B} p_d + \mathcal{C} \partial_x p_d + \mathcal{D} \partial_x^2 p_d + \mathcal{E} \partial_t p_d, \quad (\text{S65})$$

with

$$\mathcal{A} = \text{Re} \left[ \partial_z \mathcal{F} \left( \mathcal{F} + \kappa(x) \partial_x^2 z \right) + \partial_{z^*} \mathcal{F} \left( \mathcal{F} + \kappa(x) \partial_x^2 z \right)^* + \kappa(x) \partial_x^2 \left( \mathcal{F} + \kappa(x) \partial_x^2 z \right) \right], \quad (\text{S66})$$

$$\mathcal{B} = \text{Re} \left[ \frac{e^{-i\phi}}{\alpha(x)} \partial_z \mathcal{F} + \frac{e^{i\phi}}{\alpha(x)} \partial_{z^*} \mathcal{F} + \kappa(x) \partial_x^2 \left( \frac{e^{-i\phi}}{\alpha(x)} \right) \right], \quad (\text{S67})$$

$$\mathcal{C} = \text{Re} \left[ 2\kappa(x) \partial_x \left( \frac{e^{-i\phi}}{\alpha(x)} \right) \right], \quad (\text{S68})$$

$$\mathcal{D} = \text{Re} \left[ \kappa(x) \frac{e^{-i\phi}}{\alpha(x)} \right], \quad (\text{S69})$$

$$\mathcal{E} = \text{Re} \left[ \frac{e^{-i\phi}}{\alpha(x)} \right], \quad (\text{S70})$$

303 where  $\mathcal{F} = i\omega_R(x)z - (\beta_r + i\beta_i)|z|^2z$ .

304 Using Eq. (S65), we could then write Eq. (S63) as

$$p_d - 2\rho \int_0^L (\mathcal{B} p_d + \mathcal{C} \partial_{x'} p_d + \mathcal{D} \partial_{x'}^2 p_d + \mathcal{E} \partial_t p_d) g dx' = - \int_0^H P_b(y', t) \partial_{x'} G(\mathbf{r}, \mathbf{r}')|_{x'=0} dy' + 2\rho \int_0^L \mathcal{A} g dx', \quad (\text{S71})$$

305 where the left-hand side contains functions of the driving pressure  $p_d$ , while the right-hand side does  
 306 not. We recall that  $P_b$  is the stimuli at the base of the cochlea; it is related to sound-evoked pressure  
 307 in the ear canal as described in Section C4. Note that, if  $\phi = \pi/2$ , the coefficient  $\mathcal{E}$  is zero and  
 308 Eq. (S71) is independent of  $\partial_t p_d$ . In this case, the driving pressure  $p_d$  adjusts instantaneously to  
 309 time variations of fluid pressure at the base. Conversely, if  $\phi \neq \pi/2$ ,  $p_d$  at any given time depends  
 310 on its value at past times.

311 To solve numerically Eq. (S71), the  $x$ -axis was discretized into  $N_X + 1$  equally-spaced points  
 312  $\mathbf{x} = \{x_0, \dots, x_{N_X}\}$ , with a spatial step  $\Delta x = L/N_X$ . The time variable,  $t$ , was discretized by  
 313 sampling  $N_T + 1$  time points of the period,  $T = 1/f$ , of a reference frequency,  $f$ , giving a constant  
 314 time-increment of  $\Delta t = T/N_T$ . The stimulus  $P_b$  is a single tone with angular frequency  $\omega$ , see  
 315 Section C4, and the frequency  $f = \omega/(2\pi)$ . The number of cycles in a simulation is  $N_P$ , so the total  
 316 simulation time was  $N_P T$ . The continuous variables  $z(x, t)$  and  $p_d(x, t)$  were discretized in space  
 317 and time with  $z(x_j, t_n) = z_j^n$ , so at the each timestep, the following vectors were computed

$$\mathbf{z}^n = \{z_0^n, \dots, z_{N_X}^n\}, \quad (\text{S72})$$

$$\mathbf{p}_d^n = \{p_{d,0}^n, \dots, p_{d,N_X}^n\}. \quad (\text{S73})$$

318 First, at the  $n^{\text{th}}$  time step, the components of  $\mathbf{z}^n$  were computed from the values of  $\mathbf{z}$  computed  
 319 at the previous time steps ( $\mathbf{z}^{n-1}, \mathbf{z}^{n-2}, \dots$ ) using the Adams-Bashforth method on Eq. (S20)

$$z_j^n = z_j^{n-1} + \Delta t \sum_{m=0}^{m_s} a_m \text{RHS}_j^{n-1-m}, \quad (\text{S74})$$

320 where  $m_s$  is the order of the Adams-Bashforth method,  $(a_m)_{m=0, \dots, m_s}$  are the coefficients of the  
 321 Adams-Bashforth method, and RHS corresponds to the right-hand side of Eq. (S20) evaluated at  
 322 position  $x_j$  and at the  $(n-1-m)^{\text{th}}$  time step. The second-order spatial derivative in the expression  
 323 of RHS was discretized according to a central-difference scheme as

$$\partial_x^2 f \rightarrow \frac{f_{j-1} - 2f_j + f_{j+1}}{\Delta x^2} + \mathcal{O}(\Delta x^2), \quad (\text{S75})$$

324 where  $f = f(x)$  is a function of  $x$ , and  $f_j = f(x_j)$ . Boundary values of  $z$  were updated at each time  
 325 step according to the boundary conditions (S21) and (S22).

Second, the components of the driving pressure  $\mathbf{p}_d^n$  were computed by solving Eq. (S71). The components of  $\mathbf{z}^n$  were used to update the coefficients  $\mathcal{A}$  and  $\mathcal{B}$  in Eq. (S71). The second-order spatial derivatives in Eq. (S71) were discretized according to Eq. (S75). The convolution products in left-hand side of Eq. (S71) were discretized using

$$\int_0^L dx' f(x')g(x, x') \rightarrow \sum_{j=0}^{N_X} \Delta x g_{ij} f_j, \quad (\text{S76})$$

where  $g_{ij} = g(x_i, x_j)$  and  $g$  is the reduce Green function Eq. (S64). The time-derivative  $\partial_t p_d$  in Eq. (S71) was discretized as

$$\partial_t f \rightarrow \frac{f^n - f^{n-1}}{\Delta t} + \mathcal{O}(\Delta t). \quad (\text{S77})$$

and finally the integrals in the right-hand side of Eq. (S71) were computed numerically. This way the discrete version of Eq. (S71) can then be written in matrix form as

$$\mathcal{M}_{2D}(\mathbf{z}^n, (\mathbf{z}^n)^*) \mathbf{p}_d^n = \mathcal{L}_{2D}(\mathbf{z}^n, (\mathbf{z}^n)^*, \mathbf{p}_d^{n-1}). \quad (\text{S78})$$

where  $\mathcal{M}_{2D}$  is a matrix and  $\mathcal{L}_{2D}$  is the inhomogeneous term that depends on driving pressure at the previous time step. Then  $\mathbf{p}_d^n$  can be computed by inverting the relation (S78), leading to

$$\mathbf{p}_d^n = \mathcal{M}_{2D}^{-1} \mathcal{L}_{2D}(\mathbf{z}^n, (\mathbf{z}^n)^*, \mathbf{p}_d^{n-1}). \quad (\text{S79})$$

**2.b. With 1D hydrodynamics.** As with 2D hydrodynamics, we used Eq. (S65) to express  $\partial_t^2 h$  in Eq. (S40), yielding

$$-\frac{2\rho}{H} \mathcal{B} p_d - \frac{2\rho}{H} \mathcal{C} \partial_x p_d + \left(1 - \frac{2\rho}{H} \mathcal{D}\right) \partial_x^2 p_d - \frac{2\rho}{H} \mathcal{E} \partial_t p_d = \frac{2\rho}{H} \mathcal{A}(z, z^*), \quad (\text{S80})$$

where the driving pressure  $p_d(x) = p(x)$  in the limit of 1D hydrodynamics. The discretization and integration procedures in time and space were similar to those used with 2D hydrodynamics. The components of the driving pressure  $\mathbf{p}_d^n$  were computed by solving the discrete version of Eq. (S80)

$$\mathcal{M}_{1D}((\mathbf{z}^n, (\mathbf{z}^n)^*)) \mathbf{p}_d^n = \mathcal{L}_{1D}(\mathbf{z}^n, (\mathbf{z}^n)^*, \mathbf{p}_d^{n-1}), \quad (\text{S81})$$

where the matrix  $\mathcal{M}_{1D}$  and the operator  $\mathcal{L}_{1D}$  result from the discretization of Eq. (S80). Because the matrix  $\mathcal{M}_{1D}$  is sparse, in contradistinction to  $\mathcal{M}_{2D}$ , solving the model in 1D hydrodynamics is much less computationally intensive than in 2D hydrodynamics.

**2.c. Discretization of space and time.** Discretization parameters of the numerical approach ( $N_X, N_T, N_P$ ) varied within the ranges  $N_X = 100 \rightarrow 4000$ ,  $N_T = 100 \rightarrow 10000$  and  $N_P = 100 \rightarrow 2000$ . To reduce the duration of a simulation, the length of the box was adjusted to the frequency of the stimulus as  $L = 2 x_R(\omega)$ , in which  $x_R(\omega) = d \log(\omega_0/\omega)$  is the position of resonance for a pure tone of angular frequency  $\omega$ . Because  $N_X$  was fixed, the grid size  $L(\omega)/N_X$  decreased with frequency. We checked that longer boxes produced the same response. In addition, we used  $m_s = 2$  for the order of the Adams-Bashforth method with coefficients  $a_0 = 23/12$ ,  $a_1 = -4/3$ , and  $a_2 = 5/12$ . For a pure-tone stimulus of a given level, a simulation took approximately 15 min with a number of space points  $N_X = 500$ , a number of time points in a cycle  $N_T = 500$ , and number of cycles  $N_P = 100$ .

**2.d. Computation of the energy flux.** For a given cross section of the box at position  $x$ , the energy flux in the fluid is given by

$$J(x) = \int_0^H dy \langle p(x, y, t) u(x, y, t) \rangle_t, \quad (\text{S82})$$

where  $\langle \cdot \rangle_t$  denotes a time average over one period,  $2\pi/\omega$ , of the stimulus. Although one could, in principle, compute the energy flux from the full pressure field in the box, this approach is computationally expensive. Instead, we show below how to compute the energy flux from the driving pressure  $p_d(x, t) = p(x, y = 0, t)$  only.

Using hydrodynamics to relate pressure and velocity fields in the fluid (Eq. (S34)), we start by rewriting the energy flux as a function of the Fourier amplitude,  $\tilde{p}$ , at frequency  $\omega$  of the pressure field  $p(x, y, t) \simeq \tilde{p}(x, y, \omega) \exp(i\omega t) + c.c.$  as

$$J(x) = \frac{2}{\rho\omega} \int_0^H dy \operatorname{Im} [\tilde{p}(x, y, \omega) \partial_x \tilde{p}^*(x, y, \omega)]. \quad (\text{S83})$$

Note that we assume here that the Fourier component at  $\omega$  provides the dominant contribution to the energy flux.

To compute the energy flux profile  $J(x)$ , we inserted the WKB approximation of  $\tilde{p}$  (see Eq. (S86) in Section E) into Eq. (S83) with  $\partial_x \tilde{p} \simeq \frac{\cosh[q(H-y)]}{\cosh[qH]} \partial_x \tilde{p}_d(x, \omega)$ , which yields:

$$J(x, \omega) = \frac{2H}{\rho\omega} \Gamma(x, \omega) \operatorname{Im} [\tilde{p}_d(x, \omega) \partial_x \tilde{p}_d^*(x, \omega)]. \quad (\text{S84})$$

where the prefactor  $\Gamma(x, \omega)$  takes the form:

$$\Gamma(x, \omega) = \frac{1}{2qH} \left( \frac{qH}{\cosh^2(qH)} + \tanh(qH) \right). \quad (\text{S85})$$

367 The Fourier component of the driving pressure  $\tilde{p}_d(x, \omega)$  and its derivative in Eq. (S84) were  
 368 computed from the numerical solution of the model. In Eq. (S85), the wavenumber  $q$  was estimated  
 369 from the driving pressure profile  $\tilde{p}_d(x, \omega)$  as  $q \simeq \sqrt{\text{Re}(-\partial_x^2 \tilde{p}_d / \tilde{p}_d)}$ . Under the assumption of 1D  
 370 hydrodynamics ( $qH \ll 1$ ), the prefactor  $\Gamma(x, \omega)$  goes to 1.

371 **2.e. Frequency-tuning curve of sensitivity.** In the presence of mechanical coupling ( $\kappa \neq 0$  in Eq. (S20)),  
 372 the time to reach steady-state was less than 50 cycles. In this case, the simulation time was  
 373 sufficiently short (less than a day) to measure the response of the model at a fixed position as a  
 374 function of frequency,  $f$ , and level of a pure-tone stimulus,  $P_0$ . To confront the output of the model  
 375 to experiments [1], the position of measurement was set at the characteristic place,  $x = \text{CP}$ , which is  
 376 the position of maximal response at a stimulus frequency of  $f = 6.6$  kHz and a stimulus level of 10 dB.  
 377 Stimulus frequencies and levels were then varied, respectively, within a range of 660 – 10,000 Hz  
 378 with a 660-Hz increment and of 10 – 80 dB with a 10 dB increment. The frequency-tuning curves of  
 379 sensitivity were given by  $\chi(x = \text{CP}, f, P_0)$  (S50) and plotted as a function of the sound-pressure  
 380 level in decibels (Eq. (S45)).

381 In the absence of mechanical coupling ( $\kappa = 0$  in Eq. (S20)), the time to reach steady state could  
 382 reach 450 cycles at low stimulus levels. Furthermore, because the response was sharply peaked  
 383 around the characteristic place, it was also necessary to refine spatial sampling, further lengthening  
 384 the simulation time. Consequently, computing a few tuning curves could take up to one month.

385 To circumvent this technical difficulty, we used the approximation  $\chi(x, f) \simeq \chi(f/\text{CF}(x))$  with  
 386  $f/\text{CF}(x) \simeq \exp[(\text{CP}(f) - x)/d]$  following tonotopy, where CP is the characteristic place of peak  
 387 vibration at frequency  $f$ . Clearly, the approximation is exact at the peak of the response, for the  
 388 peak response is reached when  $x = \text{CP}$  and  $f = \text{CF}$ . We checked that in our simulations this  
 389 approximation remains valid near the peak—a property called local scaling invariance [25], which  
 390 allowed us to estimate the bandwidth of frequency-tuning curves with good accuracy. Then, from  
 391 a single simulation of the response profile  $\chi(x, f_{\text{STIM}})$  at a fixed stimulus frequency,  $f = f_{\text{STIM}}$ ,  
 392 we could approximate the frequency-tuning curve,  $\chi(x = \text{CP}(f_{P_{\text{STIM}}}), f)$ , at the characteristic place,  
 393  $x = \text{CP}$ , for the stimulus frequency  $f_{P_{\text{STIM}}}$  in the simulation: it is given by the parametric plot of  
 394  $\chi(x)$  as a function of  $f/\text{CF}(x) = \exp[(\text{CP}(f_{P_{\text{STIM}}}) - x)/d]$ , where position  $x$  is the parameter. We note  
 395 that the approximation of local scaling invariance does not capture the behavior of tuning curves  
 396 away from the peak, in particular the plateau of sensitivity at low frequencies; this plateau can be  
 397 estimated analytically by  $\chi(f \rightarrow 0) = G_{\text{ME}} \sin(\phi)/(\bar{\alpha}\omega_R^2)$  (see Eq. (S103)).

**3. Confronting numerical results of the model to experiments: matching procedure.** We confronted the output of the model to published experimental measurements of basilar-membrane vibrations at a fixed position within the cochlea of a chinchilla [1]. The characteristic frequency at this position was 6.6 kHz and the data consisted of 8 tuning curves corresponding to sound-pressure levels from 10 dB to 80 dB in 10 dB increments. In this section, we describe how we chose parameter values in the model.

The model comprises seven adjustable parameters:  $\bar{\alpha}$ ,  $\beta_r$ ,  $\beta_i$ ,  $\phi$ ,  $\bar{\kappa}_r$ ,  $\bar{\kappa}_i$ , and  $G_{\text{ME}}$ . The procedure consists in two steps. First, we focused on the regime of linear responsiveness at low sound-pressure levels, in which the response depends on only five parameters:  $\bar{\alpha}$ ,  $\bar{\kappa}_r$ ,  $\bar{\kappa}_i$ ,  $\phi$ ,  $G_{\text{ME}}$ . Second, we identified the pair of parameters  $(\beta_r, \beta_i)$  that control the strength of the nonlinear term in the normal form of the critical oscillators (Eq. (S20)). The parameter space was first explored using a coarse spatial discretization ( $N_X = 500$ ). Once a suitable parameter set was identified, we refined the spatial discretization to  $N_X = 3000$  to generate the tuning curves shown in the Main text.

**First step: linear-responsiveness regime** We set  $\beta = 0$  in Eq. (S20) to impose linearity and used Fourier analysis to solve the model. The output of the model was compared to experiments at a sound-pressure level of 20 dB, for which the cochlea operates in a linear regime of responsiveness [1]. For each parameter set, we computed the spatial profile of sensitivity  $\chi(x, f = f_{P_{\text{STIM}}})$  (Eq. (S50)) at the stimulus frequency  $f = f_{P_{\text{STIM}}=6.6}$  kHz. This profile peaked at a position that is called the "characteristic place" (CP). A parametric plot (parameter: position  $x$ ) of the sensitivity profile as a function of  $f/\text{CF}(x) = \exp(-(x - \text{CP})/d)$  approximated the frequency-tuning curve,  $\chi(x = \text{CP}, f)$ , measured at CP (see Section D2.e). The same transformation was used to compute the phase,  $\theta(x = \text{CP}, f)$ , of the Fourier component of the response,  $\tilde{h}(x, f)$ , at CP as a function of the frequency  $f$  of a pure-tone stimulus.

Parameters were varied using an interactive interface until the model produced frequency-tuning curves that best matched those in experiments upon visual inspection. This interface allowed real-time visualization of the frequency-tuning curves upon variation of a given parameter with a cursor. We started with parameter  $\bar{\alpha}$  to adjust the frequency dependence of the response phase  $\theta(x = \text{CP}, f)$  (Fig. S11A). Next, we adjusted the middle-ear gain,  $G_{\text{ME}}$ , which could be used to shift the tuning curve of sensitivity along the ordinate without affecting its shape nor  $\theta(x = \text{CP}, f)$ , thus affording a means to adjust the level of the low-frequency side of the tuning curve (Fig. S11B). The real part of the coupling parameter,  $\bar{\kappa}_r$ , controlled the bandwidth of sensitivity tuning curves

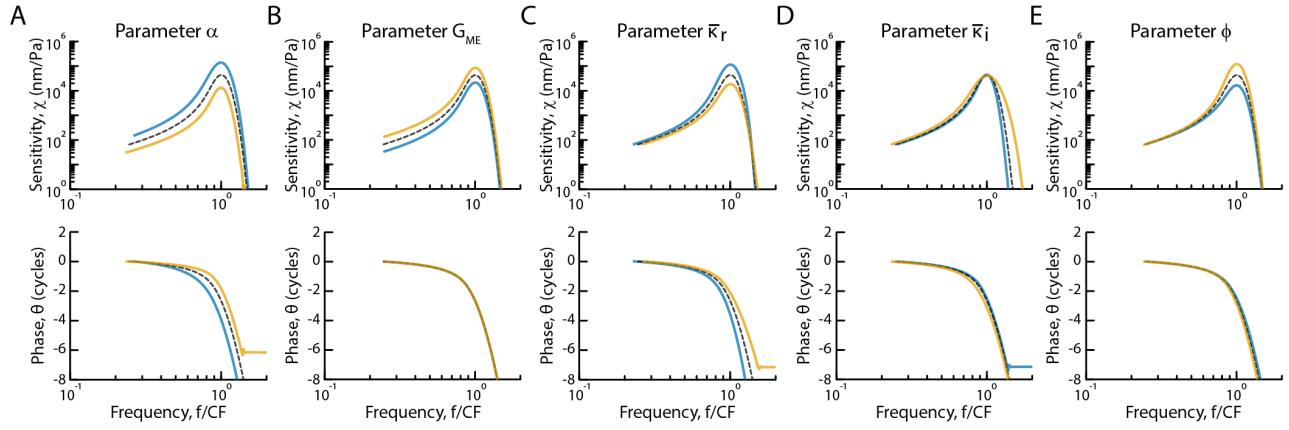

**Fig. S11.** Effects of varying parameter values on sensitivity ( $\chi$ , top row in (A-E)) and response phase ( $\theta$ , bottom row in (A-E)) as a function of stimulus frequency,  $f/CF$ , in which  $CF = 6.6$  kHz is the characteristic frequency. The dashed black lines correspond to the parameter set that we used to match experimental observations in our model with 2D hydrodynamics, viscoelastic coupling between the oscillators, and energy pumping into traveling waves (Fig.5 in the Main text with parameter values in Table S1):  $\bar{\alpha} = 0.26 \text{ Pa s}^2 \text{ m}^{-1}$ ,  $G_{ME} = 283$ ,  $\bar{\kappa}_r = 160 \mu\text{m}^2$ ,  $\bar{\kappa}_i = -160 \mu\text{m}^2$ ,  $\phi = \pi/2 - 0.4$ . We show how doubling (orange) or halving (blue) one parameter value affects the frequency profile of sensitivity and phase with respect to the reference (dashed black lines), except for parameter  $\phi$  for which we subtracted (orange) or added (blue) 0.1 rad to the reference value, corresponding to an increase or decrease of energy pumping, respectively. The frequency profiles of sensitivity and phase were computed as described in Section D2.e.

(Fig. S11C). The imaginary part of the coupling parameter,  $\bar{\kappa}_i$ , could instead be used to vary the decay rate of sensitivity beyond the peak (Fig. S11D). In the absence of coupling, there was no linear regime of responsiveness nor control over the bandwidth or the decay rate of sensitivity beyond the peak unless the oscillators were detuned from criticality ( $\varepsilon \neq 0$ ). For the later case,  $\varepsilon$  played a similar role as  $\bar{\kappa}_r$ . Finally, the phase parameter  $\phi$ , by affecting the magnitude of energy pumping, controlled the peak sensitivity (Fig. S11E). This first step of the procedure was repeated iteratively until an optimal parameter set was reached.

**Second step: Matching the model in the nonlinear responsiveness regime** Parameter  $\beta_r$  controlled the sound-pressure level of crossover between the linear and nonlinear regimes of responsiveness: lower values expanded the linear regime toward larger stimulus levels. Instead,  $\beta_i$  affected how strongly the peak in frequency-tuning curves shifted toward lower frequencies at increasing sound-pressure levels. With  $\beta_i < 0$ , the magnitude of the shift was reduced, which was associated with a change of the power-law scaling of the sensitivity at the characteristic frequency,  $\chi(x = CP, f = CF)$ , as a function of sound-pressure level in decibels (Eq. (S45)). Thus,  $\beta_i$  modulated the exponent of a power-law fit to the model in the nonlinear regime.

Without further adjustment of the parameters, the model matched, all at once, the target

experimental tuning curves and the phase at all sound-pressure levels.

**4. Parameter values and methodology for each numerical implemetation of the model (with Tables S1 and S2).** Some parameters were fixed in all realizations of our box model of the cochlea: the height of each compartment,  $H = 1$  mm, the density of the fluid in the box,  $\rho = 10^3$  kg m<sup>-3</sup> and the tonotopic map,  $\omega_R(x) = \omega_0 \exp(-x/d)$ , with  $\omega_0 = 1.89 \cdot 10^5$  rad s<sup>-1</sup> and  $d = 2.9$  mm. To reduce the duration of a simulation, the length of the box was adjusted to the frequency of the stimulus as  $L = 2 x_R(\omega)$ , in which  $x_R(\omega) = d \log(\omega_0/\omega)$  is the position of resonance for a pure tone of angular frequency  $\omega$ . The model has up to seven adjustable parameters in the normal form of a critical oscillator (Eq. (S20)):  $\bar{\varepsilon}$ ,  $\bar{\alpha}$ ,  $\bar{\beta}_r$ ,  $\bar{\beta}_i$ ,  $\phi$ ,  $\bar{\kappa}_r$ , and  $\bar{\kappa}_i$ . In practice, all the oscillators were critical ( $\varepsilon = 0$ ), except in one realization (Fig. S4) for which we imposed a distribution of control parameters that obeyed  $\varepsilon(x) = \bar{\varepsilon} \omega_R(x)$  with  $\bar{\varepsilon} \neq 0$ . We also varied the middle-ear gain,  $G_{ME}$ . Parameter values are given in Table S1 for each realization of the model, corresponding to Figures 2-6 in the Main text and Figures S2 and S4 in Section A of the Supplemental Material.

**Table S1. Parameter values for each implementation of the model.**

| Symbol                                              | Fig. 2              | Fig. 3              | Fig. 4              | Fig. 5              | Fig. 6A, S2         | Fig. 6B, 6C            | Fig. S4             |
|-----------------------------------------------------|---------------------|---------------------|---------------------|---------------------|---------------------|------------------------|---------------------|
| $\bar{\varepsilon}$                                 | 0                   | 0                   | 0                   | 0                   | 0                   | 0                      | -0.085              |
| $\bar{\alpha}$ (Pa s <sup>2</sup> m <sup>-1</sup> ) | $3.7 \cdot 10^{-1}$ | $3.7 \cdot 10^{-1}$ | $3.7 \cdot 10^{-1}$ | $2.6 \cdot 10^{-1}$ | $8.5 \cdot 10^{-2}$ | $8.5 \cdot 10^{-2}$    | $7.9 \cdot 10^{-2}$ |
| $\beta_r$ (nm <sup>-2</sup> s <sup>-1</sup> )       | 1                   | 1                   | 1                   | 9                   | 20                  | 8                      | 20                  |
| $\beta_i$ (nm <sup>-2</sup> s <sup>-1</sup> )       | 0                   | 0                   | 0                   | -6                  | 0                   | $0 \rightarrow \pi/2$  | 0                   |
| $\phi$ (rad)                                        | $\pi/2$             | $\pi/2$             | $\pi/2$             | $\pi/2 - 0.40$      | $\pi/2 - 0.75$      | $0 \rightarrow \pi/2$  | $\pi/2 - 1$         |
| $\bar{\kappa}_r$ ( $\mu$ m <sup>2</sup> )           | 0                   | 0                   | 16                  | 160                 | 260                 | $5.3 \rightarrow 5300$ | 0                   |
| $\bar{\kappa}_i$ ( $\mu$ m <sup>2</sup> )           | 0                   | 0                   | -63                 | -160                | -53                 | 0                      | 0                   |
| $G_{ME}$                                            | 283                 | 283                 | 283                 | 283                 | 95                  | 95                     | 141                 |

Table S2 also specifies, for each figure, whether the model was solved using 1D or 2D hydrodynamics and the method to compute frequency-tuning curves. Frequency-tuning curves were obtained either (label ‘A’) from a parametric plot of the sensitivity profile  $\chi(x, f = 6.6$  kHz) to a pure-tone stimulus at frequency  $f = 6.6$  kHz as a function of  $f/CF(x) = \exp(-(x - CP)/d)$ , in which CF and CP are the characteristic frequency and the characteristic place (see Section D2.e above), or (label ‘B’) from responses to pure-tone stimuli of varying frequencies at the characteristic place.

**Table S2. Methodology for each implementation of the model.**

| Method        | Fig. 2 | Fig. 3 | Fig. 4 | Fig. 5 | Fig. 6A, S2 | Fig. 6B, 6C | Fig. S4 |
|---------------|--------|--------|--------|--------|-------------|-------------|---------|
| Hydrodynamics | 1D     | 2D     | 2D     | 2D     | 1D          | 1D          | 1D      |
| Tuning curves | A      | A      | A      | B      | B           | B           | B       |

## E. Analytical solution of the model under the WKB approximation

Here, we consider the linear response and ignore mechanical coupling, corresponding to  $\beta = 0$  and  $\kappa = 0$  in Eq. (S20).

**1. Dispersion relation, pressure field and energy flux with 2D hydrodynamics.** Under the WKB approximation, as derived in the literature [17, 26], the Fourier amplitude,  $\tilde{p}$ , of the pressure field  $p(x, y, t) \simeq \tilde{p}(x, y, \omega) \exp(i\omega t) + c.c.$  evoked by a pure-tone stimulus of angular frequency  $\omega$  is given by

$$\tilde{p}(x, y, \omega) = \frac{\cosh[q(H - y)]}{\cosh[qH]} \tilde{p}_d(x, \omega), \quad (\text{S86})$$

where the Fourier amplitude,  $\tilde{p}_d$ , of the driving pressure,  $p_d(x, t) = \tilde{p}_d(x, \omega) \exp(i\omega t) + c.c.$  obeys

$$\tilde{p}_d(x, \omega) = G_{\text{ME}} P_0 \frac{q(0)H}{\tanh[q(0)H]} \left[ \frac{\frac{q(0)H}{\cosh^2[q(0)H]} + \tanh[q(0)H]}{\frac{q(x)H}{\cosh^2[q(x)H]} + \tanh[q(x)H]} \right]^{1/2} e^{-i \int_0^x dx' q(x') dx'}. \quad (\text{S87})$$

The dispersion relation

$$qH \tanh(qH) = \frac{2\rho H \omega^2}{\mathcal{A}(x, \omega)} \quad (\text{S88})$$

sets the wavenumber  $q(x, \omega)$  of the traveling wave depending on the complex modulus,  $\mathcal{A}(x, \omega)$  of the critical oscillator at position  $x$  (Eq. (S17)). Note that  $q(x, \omega)$  is here real, which implies that  $\mathcal{A}(x, \omega)$  is real and, in turn, that there is no energy pumping ( $\phi = \pi/2$ ) nor dissipation ( $\varepsilon = 0$ ). Because  $\mathcal{A}(x, \omega) = \tilde{p}_d/\tilde{h}$ , the Fourier amplitude,  $\tilde{h}$ , of the oscillator's response at position  $x$  is readily given by Equations (S17, S87 and S88).

Because  $\partial_x \tilde{p}^* \simeq i q \tilde{p}^*$ , the energy flux given by Eq.(S83) obeys the expression given by Eq. (S84) after relating  $\tilde{p}$  and  $\tilde{p}_d$  using Eq.(S86). Rewriting Eq. (S84) as

$$J(x) = \frac{qH}{\omega} \left( \frac{1}{\cosh^2(qH)} + \frac{\tanh(qH)}{qH} \right) |\tilde{p}_d(x)|^2, \quad (\text{S89})$$

we see, using Eq. (S87), that the energy flux  $J(x) = J(x = 0)$  is uniform in the absence of energy dissipation or pumping into the environment (i.e.  $q$  is real).

In the case where there is pumping or dissipation, Eqs. (S86) and (S89) still hold under the WKB approximation, but the wavenumber  $q(x, \omega)$  no longer obeys Eq. (S88). As described in Methods (Section D), the wave number is then estimated directly from the driving-pressure profile as  $q \simeq \sqrt{\text{Re}(-\partial_x^2 \tilde{p}_d / \tilde{p}_d)}$ .

**2. Dispersion relation, pressure field and energy flux with 1D hydrodynamics.** Under the assumption of 1D hydrodynamics, the pressure field is independent on the  $y$  coordinate and obeys [13, 27]

$$\partial_x^2 p = \frac{2\rho}{H} \partial_t^2 h. \quad (\text{S90})$$

In Fourier domain, using

$$\tilde{p}(x, \omega) = \mathcal{A}(x, \omega) \tilde{h}(x, \omega), \quad (\text{S91})$$

where the complex modulus  $\mathcal{A}$  is given by Eq. (S17), Eq. (S90) can be further simplified by inserting Eq. (S91) and it takes the form

$$\partial_x^2 \tilde{p}(x, \omega) = -Q^2(x, \omega) \tilde{p}(x, \omega), \quad (\text{S92})$$

where  $Q(x, \omega)$  is a complex wavenumber

$$Q^2(x, \omega) = \frac{2\rho\omega^2}{H\mathcal{A}(x, \omega)}, \quad (\text{S93})$$

Using Eq. (S17), we get the dispersion relation

$$Q^2(x, \omega) = \frac{2\rho}{\bar{\alpha}H} \frac{\bar{\omega}^2 [\sin(\phi) + i\bar{\omega} \cos(\phi)]}{1 - \bar{\omega}^2}, \quad (\text{S94})$$

where  $\bar{\omega} = \omega/\omega_R(x)$ . The real and imaginary part of  $Q^2(x, \omega) = Q_r^2(x, \omega) + iQ_i^2(x, \omega)$  take the form

$$Q_r^2(x, \omega) = \frac{2\rho}{\bar{\alpha}H} \frac{\bar{\omega}^2}{1 - \bar{\omega}^2} \sin(\phi), \quad (\text{S95})$$

$$Q_i^2(x, \omega) = \frac{2\rho}{\bar{\alpha}H} \frac{\bar{\omega}^3}{1 - \bar{\omega}^2} \cos(\phi). \quad (\text{S96})$$

To solve Eq. (S92), we consider an Ansatz corresponding to a traveling wave

$$\tilde{p}(x, \omega) = P(x, \omega) e^{-i \int_0^x q(x', \omega) dx'}, \quad (\text{S97})$$

where  $P(x, \omega)$  and  $q(x, \omega)$  determine the amplitude and phase of  $\tilde{p}(x, \omega)$ . Note that without losing generality,  $P(x, \omega)$  and  $q(x, \omega)$  can be real. Because under the WKB approximation  $\partial_x^2 P \ll q^2 P$ ,

the solution to Eq. (S92) obeys

$$P(x, \omega) = G_{\text{ME}} P_0 \sqrt{\frac{Q_r(x=0, \omega)}{Q_r(x, \omega)}} \exp\left(\frac{1}{2} \int_0^x \frac{Q_i^2(x', \omega)}{Q_r(x', \omega)} dx'\right), \quad (\text{S98})$$

$$q(x, \omega) = Q_r(x, \omega). \quad (\text{S99})$$

Using Eq. (S95), the number of cycles,  $N_R$ , that the pressure wave accumulates to reach the position of resonance ( $\bar{\omega} = 1$  or  $x = x_R$ ) is given by

$$N_R = \frac{1}{2\pi} \int_0^{x_R} q(x') dx' = \frac{d}{4} \sqrt{\frac{2\rho}{\bar{\alpha}H}} \sin(\phi). \quad (\text{S100})$$

and the argument of the exponential factor in the expression for  $P$  (Eq. (S98)) reads

$$\int_0^x \frac{Q_i^2(x', \omega)}{Q_r(x', \omega)} dx' = 4N_R \cotan(\phi) \left[1 - \sqrt{1 - \bar{\omega}^2(x)}\right]. \quad (\text{S101})$$

The amplitude of the pressure field is then

$$P(x, \omega) = G_{\text{ME}} P_0 \left( \frac{\bar{\omega}^2(x=0)}{\bar{\omega}^2(x)} \frac{1 - \bar{\omega}^2(x)}{1 - \bar{\omega}^2(x=0)} \right)^{1/4} \exp\left(2N_R \cotan(\phi) \left[1 - \sqrt{1 - \bar{\omega}^2(x)}\right]\right). \quad (\text{S102})$$

Combining Eqs. (S50, S17), the sensitivity can be expressed as

$$\chi(x, \omega) = \chi_{\emptyset} \cdot \mathcal{G}, \quad (\text{S103})$$

in which

$$\chi_{\emptyset}(x, \omega) = \frac{G_{\text{ME}}}{\bar{\alpha}\omega_R^2(x)} \left( \frac{\bar{\omega}^2(x=0)}{\bar{\omega}^2(x)(1 - \bar{\omega}^2(x=0))(1 - \bar{\omega}^2(x))^3} \right)^{1/4} \propto \frac{1}{(1 - \bar{\omega}(x))^{3/4}}, \quad (\text{S104})$$

is the sensitivity when there is no energy pumping into the traveling wave ( $\phi = \pi/2$ ) and

$$\mathcal{G}(x, \omega) = \sqrt{\sin^2(\phi) + \bar{\omega}^2(x) \cos^2(\phi)} \exp\left(2N_R \cotan(\phi) \left[1 - \sqrt{1 - \bar{\omega}^2(x)}\right]\right) \quad (\text{S105})$$

is a gain factor owing to energy pumping. In Eq. (S104), we highlighted the power-law divergence of the sensitivity as the traveling wave approaches the characteristic place where local mechanical resonance occurs ( $x \rightarrow x_R$ ,  $\bar{\omega} \rightarrow 1$ ).

Because  $\partial_x \tilde{p} \simeq -iq\tilde{p}$  under the WKB approximation, the energy flux (Eq. (S83)) can be expressed as  $J = \frac{2Hq}{\rho\omega} P^2$ . Using Eq. (S102), we get

$$J(x) = J(0) \exp\left(4N_R \cotan(\phi) \left[1 - \sqrt{1 - \bar{\omega}^2(x)}\right]\right). \quad (\text{S106})$$

Energy pumping into the traveling wave ( $\phi \neq \pi/2$ ) leads to a progressive increase of the energy flux,  $J(x) > J(0)$ , which boosts sensitivity as the wave approaches the characteristic place ( $\bar{\omega} \rightarrow 1$ ):  $\mathcal{G} \propto \sqrt{J(x)/J(0)} > 1$ . With energy pumping, sensitivity can be high before the wave reaches the characteristic place; high sensitivity does not solely rely on local resonance.

## F. Mapping between the linearized Hopf normal form and the local equation of basilar-membrane motion inferred by G. Zweig.

George Zweig has developed an inference method to derive a local equation of basilar-membrane motion from experimental measurements, which reads (Eq. (80) in Ref. [28])

$$\partial_\tau^2 y + 2\hat{\beta}_i \partial_\tau y + (\hat{\beta}_r^2 + \hat{\beta}_i^2) y = \frac{2}{\mathcal{M}\omega_c^2 \delta} \left( (r_r^\pm \hat{\beta}_r + r_i^\pm \hat{\beta}_i) p + r_i^\pm \partial_\tau p \right), \quad (\text{S107})$$

where  $\hat{\beta}_r$ ,  $\hat{\beta}_i$ ,  $\mathcal{M}$ ,  $\omega_c$ ,  $\delta$ ,  $r_r^\pm$ , and  $r_i^\pm$  are parameters, the adimensional time  $\tau = \omega_c(\chi_m)t$  is the product of time  $t$  and the characteristic frequency  $\omega_c(\chi_m)$  of peak response in a tuning curve, the variable  $y$  represents the transverse displacement of the basilar membrane, which we write  $h$  in our model, and  $p$  is the pressure across the basilar membrane, which we write  $p_d$ . For the derivation of Eq. (S107) and the physical interpretation of its parameters, we refer to Ref. [28].

This equation has the same form as the equation of motion of an active oscillator operating near a Hopf bifurcation in its linear regime of responsiveness (Eq. (S14)). By matching Eq. (S107) and Eq. (S14), one can map the parameters in these two equations:

$$\frac{\varepsilon}{\omega_R(\text{CP})} = -\hat{\beta}_i \quad (\text{S108})$$

$$\tan(\phi) = \frac{r_r^\pm \hat{\beta}_r}{r_i^\pm}. \quad (\text{S109})$$

Using the parameter values  $\hat{\beta}_r = 0.979$ ,  $\hat{\beta}_i = 0.0282$ ,  $r_r^\pm = 4.52$  and  $r_i^\pm = 4.76$  from Ref. [28], we get  $\varepsilon/\omega_R(\text{CP}) = -0.03$  and  $\phi = 0.75 \text{ rad} \approx \pi/4$ . Thus, the local oscillator inferred by G. Zweig is equivalent to a critical oscillator operating in a linear regime of responsiveness when it is slightly detuned from the critical point ( $|\varepsilon/\omega_R| \ll 1$ ) and provides energy pumping into the environment ( $\phi \neq \pi/2$ ) when driven below its natural frequency  $\omega_R$ .

## References

1. WS Rhode, Basilar membrane mechanics in the 6–9kHz region of sensitive chinchilla cochleae. *The J. Acoust. Soc. Am.* **121**, 2792–2804 (2007).
2. JB Dewey, CA Shera, Bandpass Shape of Distortion-Product Otoacoustic Emission Ratio Functions Reflects Cochlear Frequency Tuning in Normal-Hearing Mice. *J. Assoc. for Res. Otolaryngol.* **24**, 305–324 (2023).
3. JD Crawford, Introduction to bifurcation theory. *Rev. Mod. Phys.* **63**, 991–1037 (1991).

- 539 4. ST Strogatz, *Nonlinear Dynamics and Chaos*. (Addison-Wesley, Reading, MA), 7th edition,  
540 (1997).
- 541 5. S Camalet, T Duke, F Jülicher, J Prost, Auditory sensitivity provided by self-tuned critical  
542 oscillations of hair cells. *Proc. Natl. Acad. Sci.* **97**, 3183–3188 (2000).
- 543 6. F Jülicher, D Andor, T Duke, Physical basis of two-tone interference in hearing. *Proc. Natl.*  
544 *Acad. Sci.* **98**, 9080–9085 (2001).
- 545 7. TA Duke, F Jülicher, Critical Oscillators as Active Elements in Hearing in *Active Processes*  
546 *and Otoacoustic Emissions in Hearing*, eds. GA Manley, RR Fay, AN Popper. (Springer New  
547 York, New York, NY), pp. 63–92 (2008).
- 548 8. F Jülicher, K Dierkes, B Lindner, J Prost, P Martin, Spontaneous movements and linear  
549 response of a noisy oscillator. *The Eur. Phys. J. E* **29**, 449–460 (2009).
- 550 9. P Martin, GA Manley, *Auditory processing by the cochlea*. (2021) Publisher: McGraw-Hill  
551 Education/Medical; 6th edition.
- 552 10. AJ Hudspeth, P Martin, The Critical Thing about the Ear’s Sensory Hair Cells. *J. Neurosci.*  
553 **44** (2024) Publisher: Society for Neuroscience Section: Viewpoints.
- 554 11. AJ Hudspeth, F Jülicher, P Martin, A Critique of the Critical Cochlea: Hopf—a Bifurcation—Is  
555 Better Than None. *J. Neurophysiol.* **104**, 1219–1229 (2010).
- 556 12. F Fruth, F Jülicher, B Lindner, An Active Oscillator Model Describes the Statistics of Sponta-  
557 neous Otoacoustic Emissions. *Biophys. J.* **107**, 815–824 (2014).
- 558 13. T Duke, F Jülicher, Active Traveling Wave in the Cochlea. *Phys. Rev. Lett.* **90**, 158101 (2003).
- 559 14. MA Ruggero, AN Temchin, The roles of the external, middle, and inner ears in determining  
560 the bandwidth of hearing. *Proc. Natl. Acad. Sci. United States Am.* **99**, 13206–13210 (2002).
- 561 15. R Aibara, JT Welsh, S Puria, RL Goode, Human middle-ear sound transfer function and  
562 cochlear input impedance. *Hear. Res* **152**, 100–9 (2001).
- 563 16. ME Ravicz, MC Slama, JJ Rosowski, Middle-ear pressure gain and cochlear partition differential  
564 pressure in chinchilla. *Hear. Res.* **263**, 16–25 (2010).
- 565 17. M Viergever, Doctoral thesis (Delft University of Technology) (1980).
- 566 18. H Duifhuis, CA Shera, ES Olson, Hopf-Bifurcations and Van der Pol Oscillator Models of the  
567 Mammalian Cochlea. (Williamstown, Massachusetts (USA)), pp. 199–205 (2011).
- 568 19. JD Jackson, *Classical electrodynamics*. (John Wiley & Sons), (2021).
- 569 20. JB Allen, Two-dimensional cochlear fluid model: New results. *The J. Acoust. Soc. Am.* **61**,

110–119 (1977).

21. F Mammano, R Nobili, Biophysics of the cochlea: Linear approximation. *J. Acoust. Soc. Am.* **93**, 14 (1993).
22. CA Shera, A Tubis, CL Talmadge, Coherent reflection in a two-dimensional cochlea: Short-wave versus long-wave scattering in the generation of reflection-source otoacoustic emissions. *The J. Acoust. Soc. Am.* **118**, 287–313 (2005).
23. J Cuenca, F Gautier, L Simon, The image source method for calculating the vibrations of simply supported convex polygonal plates. *J. Sound Vib.* **322**, 1048–1069 (2009).
24. H Ver Hulst, Ph.D. thesis (Université Paris Sciences & Lettres) (2024).
25. G Zweig, Basilar Membrane Motion. *Cold Spring Harb. Symp. on Quant. Biol.* **40**, 619–633 (1976).
26. H Duifhuis, *Cochlear Mechanics*. (Springer US, Boston, MA), (2012).
27. J Lighthill, Energy flow in the cochlea. *J. Fluid Mech.* **106**, 149 (1981).
28. G Zweig, Linear cochlear mechanics. *The J. Acoust. Soc. Am.* **138**, 1102–1121 (2015).
